# Supplementary material for: Consent in Crisis: The Rapid Decline of the AI Data Commons
Source: arXiv:2407.14933 source file (2024-07-24)
Supplement: Supplementary file 1 [file appendix.tex]

% these are really really long and we should put them at the end
\section{Datasets}
\label{app:datasets}
This section provides a detailed overview of the datasets we have collected and analyzed. \Cref{tab:collections-text} summarizes the text datasets, \Cref{tab:collections-audio} the audio datasets, and \Cref{tab:collections-video} the video datasets. Each of these tables lists broad collections of data, sorted in chronological order, and provides information about their properties, sizes, sources and permissions. Each collection can include multiple datasets, and they generally reflect the ways dataset creators have grouped their datasets (such as in the same paper).

% we've commented these tables out below because they're huge and they have 30 pages of references -- fix the warnings by turning them back on
We go into more detail on the licenses of each data collection and its constituent datasets in \Cref{tab:refs-licenses-text} (for text), \Cref{tab:refs-licenses-audio} (for audio), \Cref{tab:refs-licenses-video} (for video). These latter tables also cite all of the papers which introduced our various collections (284 in all).

\setlength{\tabcolsep}{1.9pt}
\definecolor{colorRiddleSensePropertyCounts_Datasets}{RGB}{240,223,178}
\definecolor{colorFeedbackColl.PropertyCounts_Datasets}{RGB}{240,223,178}
\definecolor{colorNectarPropertyCounts_Datasets}{RGB}{240,223,178}
\definecolor{colorMetaMathQAPropertyCounts_Datasets}{RGB}{245,244,242}
\definecolor{colorMegaWikaPropertyCounts_Datasets}{RGB}{200,234,229}
\definecolor{colorOpenGPTHealthcarePropertyCounts_Datasets}{RGB}{245,236,212}
\definecolor{colorMedInstr.PropertyCounts_Datasets}{RGB}{240,223,178}
\definecolor{colorMathInstr.PropertyCounts_Datasets}{RGB}{240,223,178}
\definecolor{colorMathDialPropertyCounts_Datasets}{RGB}{240,223,178}
\definecolor{colorUltraFeedbackArgillaPropertyCounts_Datasets}{RGB}{245,244,244}
\definecolor{colorLMSYS-Chat-1MPropertyCounts_Datasets}{RGB}{240,223,178}
\definecolor{colorPII-Masking-200kPropertyCounts_Datasets}{RGB}{240,223,178}
\definecolor{colorHelpSteerPropertyCounts_Datasets}{RGB}{240,223,178}
\definecolor{colorPure-DovePropertyCounts_Datasets}{RGB}{240,223,178}
\definecolor{colorGlaiveCodeAsst.PropertyCounts_Datasets}{RGB}{240,223,178}
\definecolor{colorNoRobotsPropertyCounts_Datasets}{RGB}{240,223,178}
\definecolor{colorOpenAsst.v2PropertyCounts_Datasets}{RGB}{226,240,238}
\definecolor{colorEverythingLMPropertyCounts_Datasets}{RGB}{240,223,178}
\definecolor{colorUltraChat-200kPropertyCounts_Datasets}{RGB}{240,223,178}
\definecolor{colorThaiGenAIPropertyCounts_Datasets}{RGB}{245,244,244}
\definecolor{colorBactrian-XPropertyCounts_Datasets}{RGB}{245,241,232}
\definecolor{colorCOBRAFramesPropertyCounts_Datasets}{RGB}{240,223,178}
\definecolor{colorSelFeePropertyCounts_Datasets}{RGB}{240,223,178}
\definecolor{colorCapybaraPropertyCounts_Datasets}{RGB}{240,243,243}
\definecolor{colorExpertQAPropertyCounts_Datasets}{RGB}{240,223,178}
\definecolor{colorChatDoctorPropertyCounts_Datasets}{RGB}{245,236,212}
\definecolor{colorSeaBenchPropertyCounts_Datasets}{RGB}{245,244,244}
\definecolor{colorCollectiveCognitionPropertyCounts_Datasets}{RGB}{240,223,178}
\definecolor{colorDeita10KPropertyCounts_Datasets}{RGB}{245,234,202}
\definecolor{colorPygmalionAI-PIPPAPropertyCounts_Datasets}{RGB}{240,223,178}
\definecolor{colorChatbotArenaPropertyCounts_Datasets}{RGB}{240,223,178}
\definecolor{colorOpenMathInstr.-1PropertyCounts_Datasets}{RGB}{245,234,202}
\definecolor{colorOrca-MathPropertyCounts_Datasets}{RGB}{240,223,178}
\definecolor{color10kPromptRankedPropertyCounts_Datasets}{RGB}{240,223,178}
\definecolor{colorLongAlign-10kPropertyCounts_Datasets}{RGB}{240,223,178}
\definecolor{colorLlama2-MedTuned-Instr.PropertyCounts_Datasets}{RGB}{240,223,178}
\definecolor{colorKIWIPropertyCounts_Datasets}{RGB}{240,223,178}
\definecolor{colorIndic-Instr.PropertyCounts_Datasets}{RGB}{245,244,242}
\definecolor{colorGretelText-to-SQLPropertyCounts_Datasets}{RGB}{240,223,178}
\definecolor{colorConiferPropertyCounts_Datasets}{RGB}{240,223,178}
\definecolor{colorCidarPropertyCounts_Datasets}{RGB}{240,223,178}
\definecolor{colorAyaPropertyCounts_Datasets}{RGB}{187,229,223}
\definecolor{colorWildChatPropertyCounts_Datasets}{RGB}{245,234,202}
\definecolor{colorMedicalMeadowPropertyCounts_Datasets}{RGB}{245,244,242}
\definecolor{colorPMC-LLaMAInstr.PropertyCounts_Datasets}{RGB}{245,243,238}
\definecolor{colorDialogStudioPropertyCounts_Datasets}{RGB}{179,226,219}
\definecolor{colorCOIGPropertyCounts_Datasets}{RGB}{227,240,239}
\definecolor{colorAgentInstructPropertyCounts_Datasets}{RGB}{245,241,232}
\definecolor{colorOpen-PlatypusPropertyCounts_Datasets}{RGB}{242,244,244}
\definecolor{colorRiddleSensePropertyCounts_Tasks}{RGB}{245,241,230}
\definecolor{colorFeedbackColl.PropertyCounts_Tasks}{RGB}{245,236,212}
\definecolor{colorNectarPropertyCounts_Tasks}{RGB}{240,223,178}
\definecolor{colorMetaMathQAPropertyCounts_Tasks}{RGB}{245,236,212}
\definecolor{colorMegaWikaPropertyCounts_Tasks}{RGB}{240,223,178}
\definecolor{colorOpenGPTHealthcarePropertyCounts_Tasks}{RGB}{245,244,244}
\definecolor{colorMedInstr.PropertyCounts_Tasks}{RGB}{240,223,178}
\definecolor{colorMathInstr.PropertyCounts_Tasks}{RGB}{245,241,230}
\definecolor{colorMathDialPropertyCounts_Tasks}{RGB}{245,236,212}
\definecolor{colorUltraFeedbackArgillaPropertyCounts_Tasks}{RGB}{185,228,221}
\definecolor{colorLMSYS-Chat-1MPropertyCounts_Tasks}{RGB}{213,237,234}
\definecolor{colorPII-Masking-200kPropertyCounts_Tasks}{RGB}{245,236,212}
\definecolor{colorHelpSteerPropertyCounts_Tasks}{RGB}{236,243,242}
\definecolor{colorPure-DovePropertyCounts_Tasks}{RGB}{245,244,244}
\definecolor{colorGlaiveCodeAsst.PropertyCounts_Tasks}{RGB}{245,236,212}
\definecolor{colorNoRobotsPropertyCounts_Tasks}{RGB}{218,238,235}
\definecolor{colorOpenAsst.v2PropertyCounts_Tasks}{RGB}{245,244,244}
\definecolor{colorEverythingLMPropertyCounts_Tasks}{RGB}{218,238,235}
\definecolor{colorUltraChat-200kPropertyCounts_Tasks}{RGB}{224,240,237}
\definecolor{colorThaiGenAIPropertyCounts_Tasks}{RGB}{204,235,230}
\definecolor{colorBactrian-XPropertyCounts_Tasks}{RGB}{245,244,244}
\definecolor{colorCOBRAFramesPropertyCounts_Tasks}{RGB}{240,223,178}
\definecolor{colorSelFeePropertyCounts_Tasks}{RGB}{236,243,242}
\definecolor{colorCapybaraPropertyCounts_Tasks}{RGB}{179,226,219}
\definecolor{colorExpertQAPropertyCounts_Tasks}{RGB}{245,241,230}
\definecolor{colorChatDoctorPropertyCounts_Tasks}{RGB}{240,223,178}
\definecolor{colorSeaBenchPropertyCounts_Tasks}{RGB}{245,244,244}
\definecolor{colorCollectiveCognitionPropertyCounts_Tasks}{RGB}{229,241,239}
\definecolor{colorDeita10KPropertyCounts_Tasks}{RGB}{204,235,230}
\definecolor{colorPygmalionAI-PIPPAPropertyCounts_Tasks}{RGB}{245,241,230}
\definecolor{colorChatbotArenaPropertyCounts_Tasks}{RGB}{245,244,244}
\definecolor{colorOpenMathInstr.-1PropertyCounts_Tasks}{RGB}{245,241,230}
\definecolor{colorOrca-MathPropertyCounts_Tasks}{RGB}{240,223,178}
\definecolor{color10kPromptRankedPropertyCounts_Tasks}{RGB}{199,234,229}
\definecolor{colorLongAlign-10kPropertyCounts_Tasks}{RGB}{245,241,230}
\definecolor{colorLlama2-MedTuned-Instr.PropertyCounts_Tasks}{RGB}{245,244,244}
\definecolor{colorKIWIPropertyCounts_Tasks}{RGB}{240,223,178}
\definecolor{colorIndic-Instr.PropertyCounts_Tasks}{RGB}{224,240,237}
\definecolor{colorGretelText-to-SQLPropertyCounts_Tasks}{RGB}{240,223,178}
\definecolor{colorConiferPropertyCounts_Tasks}{RGB}{218,238,235}
\definecolor{colorCidarPropertyCounts_Tasks}{RGB}{218,238,235}
\definecolor{colorAyaPropertyCounts_Tasks}{RGB}{224,240,237}
\definecolor{colorWildChatPropertyCounts_Tasks}{RGB}{224,240,237}
\definecolor{colorMedicalMeadowPropertyCounts_Tasks}{RGB}{245,236,212}
\definecolor{colorPMC-LLaMAInstr.PropertyCounts_Tasks}{RGB}{240,223,178}
\definecolor{colorDialogStudioPropertyCounts_Tasks}{RGB}{245,241,230}
\definecolor{colorCOIGPropertyCounts_Tasks}{RGB}{199,234,229}
\definecolor{colorAgentInstructPropertyCounts_Tasks}{RGB}{245,241,230}
\definecolor{colorOpen-PlatypusPropertyCounts_Tasks}{RGB}{208,236,232}
\definecolor{colorRiddleSensePropertyCounts_Langs}{RGB}{240,223,178}
\definecolor{colorFeedbackColl.PropertyCounts_Langs}{RGB}{240,223,178}
\definecolor{colorNectarPropertyCounts_Langs}{RGB}{240,223,178}
\definecolor{colorMetaMathQAPropertyCounts_Langs}{RGB}{240,223,178}
\definecolor{colorMegaWikaPropertyCounts_Langs}{RGB}{196,232,227}
\definecolor{colorOpenGPTHealthcarePropertyCounts_Langs}{RGB}{240,223,178}
\definecolor{colorMedInstr.PropertyCounts_Langs}{RGB}{240,223,178}
\definecolor{colorMathInstr.PropertyCounts_Langs}{RGB}{240,223,178}
\definecolor{colorMathDialPropertyCounts_Langs}{RGB}{240,223,178}
\definecolor{colorUltraFeedbackArgillaPropertyCounts_Langs}{RGB}{240,223,178}
\definecolor{colorLMSYS-Chat-1MPropertyCounts_Langs}{RGB}{245,241,230}
\definecolor{colorPII-Masking-200kPropertyCounts_Langs}{RGB}{245,239,222}
\definecolor{colorHelpSteerPropertyCounts_Langs}{RGB}{240,223,178}
\definecolor{colorPure-DovePropertyCounts_Langs}{RGB}{240,223,178}
\definecolor{colorGlaiveCodeAsst.PropertyCounts_Langs}{RGB}{245,234,202}
\definecolor{colorNoRobotsPropertyCounts_Langs}{RGB}{240,223,178}
\definecolor{colorOpenAsst.v2PropertyCounts_Langs}{RGB}{222,239,237}
\definecolor{colorEverythingLMPropertyCounts_Langs}{RGB}{245,234,202}
\definecolor{colorUltraChat-200kPropertyCounts_Langs}{RGB}{240,223,178}
\definecolor{colorThaiGenAIPropertyCounts_Langs}{RGB}{240,223,178}
\definecolor{colorBactrian-XPropertyCounts_Langs}{RGB}{245,242,234}
\definecolor{colorCOBRAFramesPropertyCounts_Langs}{RGB}{240,223,178}
\definecolor{colorSelFeePropertyCounts_Langs}{RGB}{240,223,178}
\definecolor{colorCapybaraPropertyCounts_Langs}{RGB}{245,234,202}
\definecolor{colorExpertQAPropertyCounts_Langs}{RGB}{240,223,178}
\definecolor{colorChatDoctorPropertyCounts_Langs}{RGB}{240,223,178}
\definecolor{colorSeaBenchPropertyCounts_Langs}{RGB}{244,244,244}
\definecolor{colorCollectiveCognitionPropertyCounts_Langs}{RGB}{240,223,178}
\definecolor{colorDeita10KPropertyCounts_Langs}{RGB}{240,223,178}
\definecolor{colorPygmalionAI-PIPPAPropertyCounts_Langs}{RGB}{240,223,178}
\definecolor{colorChatbotArenaPropertyCounts_Langs}{RGB}{240,223,178}
\definecolor{colorOpenMathInstr.-1PropertyCounts_Langs}{RGB}{240,223,178}
\definecolor{colorOrca-MathPropertyCounts_Langs}{RGB}{240,223,178}
\definecolor{color10kPromptRankedPropertyCounts_Langs}{RGB}{240,223,178}
\definecolor{colorLongAlign-10kPropertyCounts_Langs}{RGB}{240,223,178}
\definecolor{colorLlama2-MedTuned-Instr.PropertyCounts_Langs}{RGB}{240,223,178}
\definecolor{colorKIWIPropertyCounts_Langs}{RGB}{240,223,178}
\definecolor{colorIndic-Instr.PropertyCounts_Langs}{RGB}{245,234,202}
\definecolor{colorGretelText-to-SQLPropertyCounts_Langs}{RGB}{245,237,214}
\definecolor{colorConiferPropertyCounts_Langs}{RGB}{240,223,178}
\definecolor{colorCidarPropertyCounts_Langs}{RGB}{240,223,178}
\definecolor{colorAyaPropertyCounts_Langs}{RGB}{179,226,219}
\definecolor{colorWildChatPropertyCounts_Langs}{RGB}{240,243,243}
\definecolor{colorMedicalMeadowPropertyCounts_Langs}{RGB}{240,223,178}
\definecolor{colorPMC-LLaMAInstr.PropertyCounts_Langs}{RGB}{240,223,178}
\definecolor{colorDialogStudioPropertyCounts_Langs}{RGB}{245,241,230}
\definecolor{colorCOIGPropertyCounts_Langs}{RGB}{245,234,202}
\definecolor{colorAgentInstructPropertyCounts_Langs}{RGB}{240,223,178}
\definecolor{colorOpen-PlatypusPropertyCounts_Langs}{RGB}{206,235,231}
\definecolor{colorRiddleSensePropertyCounts_Domains}{RGB}{240,223,178}
\definecolor{colorFeedbackColl.PropertyCounts_Domains}{RGB}{240,223,178}
\definecolor{colorNectarPropertyCounts_Domains}{RGB}{245,236,210}
\definecolor{colorMetaMathQAPropertyCounts_Domains}{RGB}{240,223,178}
\definecolor{colorMegaWikaPropertyCounts_Domains}{RGB}{240,223,178}
\definecolor{colorOpenGPTHealthcarePropertyCounts_Domains}{RGB}{240,223,178}
\definecolor{colorMedInstr.PropertyCounts_Domains}{RGB}{240,223,178}
\definecolor{colorMathInstr.PropertyCounts_Domains}{RGB}{240,223,178}
\definecolor{colorMathDialPropertyCounts_Domains}{RGB}{245,243,238}
\definecolor{colorUltraFeedbackArgillaPropertyCounts_Domains}{RGB}{185,228,221}
\definecolor{colorLMSYS-Chat-1MPropertyCounts_Domains}{RGB}{240,223,178}
\definecolor{colorPII-Masking-200kPropertyCounts_Domains}{RGB}{240,223,178}
\definecolor{colorHelpSteerPropertyCounts_Domains}{RGB}{240,223,178}
\definecolor{colorPure-DovePropertyCounts_Domains}{RGB}{240,223,178}
\definecolor{colorGlaiveCodeAsst.PropertyCounts_Domains}{RGB}{240,223,178}
\definecolor{colorNoRobotsPropertyCounts_Domains}{RGB}{240,223,178}
\definecolor{colorOpenAsst.v2PropertyCounts_Domains}{RGB}{240,223,178}
\definecolor{colorEverythingLMPropertyCounts_Domains}{RGB}{240,223,178}
\definecolor{colorUltraChat-200kPropertyCounts_Domains}{RGB}{245,236,210}
\definecolor{colorThaiGenAIPropertyCounts_Domains}{RGB}{240,223,178}
\definecolor{colorBactrian-XPropertyCounts_Domains}{RGB}{240,223,178}
\definecolor{colorCOBRAFramesPropertyCounts_Domains}{RGB}{245,236,210}
\definecolor{colorSelFeePropertyCounts_Domains}{RGB}{240,223,178}
\definecolor{colorCapybaraPropertyCounts_Domains}{RGB}{240,223,178}
\definecolor{colorExpertQAPropertyCounts_Domains}{RGB}{240,223,178}
\definecolor{colorChatDoctorPropertyCounts_Domains}{RGB}{245,236,210}
\definecolor{colorSeaBenchPropertyCounts_Domains}{RGB}{242,244,244}
\definecolor{colorCollectiveCognitionPropertyCounts_Domains}{RGB}{240,223,178}
\definecolor{colorDeita10KPropertyCounts_Domains}{RGB}{245,240,226}
\definecolor{colorPygmalionAI-PIPPAPropertyCounts_Domains}{RGB}{240,223,178}
\definecolor{colorChatbotArenaPropertyCounts_Domains}{RGB}{240,223,178}
\definecolor{colorOpenMathInstr.-1PropertyCounts_Domains}{RGB}{245,240,226}
\definecolor{colorOrca-MathPropertyCounts_Domains}{RGB}{245,240,226}
\definecolor{color10kPromptRankedPropertyCounts_Domains}{RGB}{245,243,238}
\definecolor{colorLongAlign-10kPropertyCounts_Domains}{RGB}{240,223,178}
\definecolor{colorLlama2-MedTuned-Instr.PropertyCounts_Domains}{RGB}{240,223,178}
\definecolor{colorKIWIPropertyCounts_Domains}{RGB}{245,236,210}
\definecolor{colorIndic-Instr.PropertyCounts_Domains}{RGB}{245,240,226}
\definecolor{colorGretelText-to-SQLPropertyCounts_Domains}{RGB}{240,223,178}
\definecolor{colorConiferPropertyCounts_Domains}{RGB}{245,236,210}
\definecolor{colorCidarPropertyCounts_Domains}{RGB}{240,223,178}
\definecolor{colorAyaPropertyCounts_Domains}{RGB}{240,223,178}
\definecolor{colorWildChatPropertyCounts_Domains}{RGB}{240,223,178}
\definecolor{colorMedicalMeadowPropertyCounts_Domains}{RGB}{245,240,226}
\definecolor{colorPMC-LLaMAInstr.PropertyCounts_Domains}{RGB}{245,236,210}
\definecolor{colorDialogStudioPropertyCounts_Domains}{RGB}{245,240,226}
\definecolor{colorCOIGPropertyCounts_Domains}{RGB}{179,226,219}
\definecolor{colorAgentInstructPropertyCounts_Domains}{RGB}{229,241,239}
\definecolor{colorOpen-PlatypusPropertyCounts_Domains}{RGB}{224,240,237}

\begin{longtable}{lc|cccc|c|cc}
\caption[\textbf{Alignment tuning (text) collections and properties}]{\textbf{Alignment tuning (text) collections and properties}. Collection properties include numbers of datasets, tasks, languages, and text domains. The \textsc{Source} column indicates whether a collection contains human-generated web text (\emoji{globe-with-meridians}), language model outputs (\emoji{robot}) or both (\emoji{globe-with-meridians}\emoji{robot}). The \textsc{Use} column indicates whether a collection includes data freely usable even for commercial purposes (\protect\CommercialDataCircle), data usable only for noncommercial purposes or academic research (\protect\NCDataCircle) and data whose license status is not specified precisely enough to allow us to determine commercial use permissions (\protect\UnspecifiedDataCircle). Note that each collection may have different datasets with one, two, or all three of these statuses. Finally, the \textsc{OAI} column indicates collections which include OpenAI model generations. Datasets are sorted chronologically to highlight trends over time.} \label{tab:collections-text} \\
\toprule
\textsc{Collection} & \textsc{} & \multicolumn{4}{c}{\textsc{Property Counts}} & \textsc{Types} & \multicolumn{2}{c}{\textsc{Permissions}} \\
 & \textsc{\thead{Year}} & \textsc{\thead{Datasets}} & \textsc{\thead{Tasks}} & \textsc{\thead{Langs}} & \textsc{\thead{Domains}} & \textsc{\thead{Source}} & \textsc{\thead{Use}} & \textsc{\thead{OAI}} \\
\midrule
\endfirsthead
\caption[]{\textbf{Alignment tuning (text) collections and properties}.} \\
\toprule
\textsc{Collection} & \textsc{} & \multicolumn{4}{c}{\textsc{Property Counts}} & \textsc{Types} & \multicolumn{2}{c}{\textsc{Permissions}} \\
 & \textsc{\thead{Year}} & \textsc{\thead{Datasets}} & \textsc{\thead{Tasks}} & \textsc{\thead{Langs}} & \textsc{\thead{Domains}} & \textsc{\thead{Source}} & \textsc{\thead{Use}} & \textsc{\thead{OAI}} \\
\midrule
\endhead
\midrule
\multicolumn{9}{r}{Continued on next page} \\
\midrule
\endfoot
\bottomrule
\endlastfoot
RiddleSense & 2021 & \cellcolor{colorCidarPropertyCounts_Datasets}{1} & \cellcolor{colorAgentInstructPropertyCounts_Tasks}{3} & \cellcolor{colorAgentInstructPropertyCounts_Langs}{1} & \cellcolor{colorWildChatPropertyCounts_Domains}{1} & \emoji{globe-with-meridians}\emojiblank & \CommercialDataCircle \TransparentCircle \TransparentCircle & \emojiblank \\
Feedback Coll. & 2023 & \cellcolor{colorCidarPropertyCounts_Datasets}{1} & \cellcolor{colorMedicalMeadowPropertyCounts_Tasks}{2} & \cellcolor{colorAgentInstructPropertyCounts_Langs}{1} & \cellcolor{colorWildChatPropertyCounts_Domains}{1} & \emojiblank\emoji{robot} & \CommercialDataCircle \TransparentCircle \TransparentCircle & \greencheck \\
Nectar & 2023 & \cellcolor{colorCidarPropertyCounts_Datasets}{1} & \cellcolor{colorPMC-LLaMAInstr.PropertyCounts_Tasks}{1} & \cellcolor{colorAgentInstructPropertyCounts_Langs}{1} & \cellcolor{colorPMC-LLaMAInstr.PropertyCounts_Domains}{2} & \emojiblank\emoji{robot} & \CommercialDataCircle \TransparentCircle \NCDataCircle & \greencheck \\
MetaMathQA & 2023 & \cellcolor{colorMedicalMeadowPropertyCounts_Datasets}{8} & \cellcolor{colorMedicalMeadowPropertyCounts_Tasks}{2} & \cellcolor{colorAgentInstructPropertyCounts_Langs}{1} & \cellcolor{colorWildChatPropertyCounts_Domains}{1} & \emojiblank\emoji{robot} & \CommercialDataCircle \TransparentCircle \TransparentCircle & \greencheck \\
MegaWika & 2023 & \cellcolor{colorMegaWikaPropertyCounts_Datasets}{50} & \cellcolor{colorPMC-LLaMAInstr.PropertyCounts_Tasks}{1} & \cellcolor{colorMegaWikaPropertyCounts_Langs}{50} & \cellcolor{colorWildChatPropertyCounts_Domains}{1} & \emojiblank\emoji{robot} & \CommercialDataCircle \TransparentCircle \TransparentCircle & \emojiblank \\
OpenGPT Healthcare & 2023 & \cellcolor{colorChatDoctorPropertyCounts_Datasets}{3} & \cellcolor{colorLlama2-MedTuned-Instr.PropertyCounts_Tasks}{4} & \cellcolor{colorAgentInstructPropertyCounts_Langs}{1} & \cellcolor{colorWildChatPropertyCounts_Domains}{1} & \emojiblank\emoji{robot} & \CommercialDataCircle \UnspecifiedDataCircle \TransparentCircle & \greencheck \\
MedInstr. & 2023 & \cellcolor{colorCidarPropertyCounts_Datasets}{1} & \cellcolor{colorPMC-LLaMAInstr.PropertyCounts_Tasks}{1} & \cellcolor{colorAgentInstructPropertyCounts_Langs}{1} & \cellcolor{colorWildChatPropertyCounts_Domains}{1} & \emojiblank\emoji{robot} & \TransparentCircle \UnspecifiedDataCircle \TransparentCircle & \greencheck \\
MathInstr. & 2023 & \cellcolor{colorCidarPropertyCounts_Datasets}{1} & \cellcolor{colorAgentInstructPropertyCounts_Tasks}{3} & \cellcolor{colorAgentInstructPropertyCounts_Langs}{1} & \cellcolor{colorWildChatPropertyCounts_Domains}{1} & \emojiblank\emoji{robot} & \CommercialDataCircle \TransparentCircle \TransparentCircle & \greencheck \\
MathDial & 2023 & \cellcolor{colorCidarPropertyCounts_Datasets}{1} & \cellcolor{colorMedicalMeadowPropertyCounts_Tasks}{2} & \cellcolor{colorAgentInstructPropertyCounts_Langs}{1} & \cellcolor{color10kPromptRankedPropertyCounts_Domains}{4} & \emojiblank\emoji{robot} & \CommercialDataCircle \TransparentCircle \TransparentCircle & \greencheck \\
UltraFeedback Argilla & 2023 & \cellcolor{colorSeaBenchPropertyCounts_Datasets}{9} & \cellcolor{colorUltraFeedbackArgillaPropertyCounts_Tasks}{16} & \cellcolor{colorAgentInstructPropertyCounts_Langs}{1} & \cellcolor{colorUltraFeedbackArgillaPropertyCounts_Domains}{20} & \emoji{globe-with-meridians}\emoji{robot} & \CommercialDataCircle \UnspecifiedDataCircle \NCDataCircle & \greencheck \\
LMSYS-Chat-1M & 2023 & \cellcolor{colorCidarPropertyCounts_Datasets}{1} & \cellcolor{colorLMSYS-Chat-1MPropertyCounts_Tasks}{9} & \cellcolor{colorDialogStudioPropertyCounts_Langs}{5} & \cellcolor{colorWildChatPropertyCounts_Domains}{1} & \emojiblank\emoji{robot} & \CommercialDataCircle \TransparentCircle \NCDataCircle & \greencheck \\
PII-Masking-200k & 2023 & \cellcolor{colorCidarPropertyCounts_Datasets}{1} & \cellcolor{colorMedicalMeadowPropertyCounts_Tasks}{2} & \cellcolor{colorPII-Masking-200kPropertyCounts_Langs}{4} & \cellcolor{colorWildChatPropertyCounts_Domains}{1} & \emoji{globe-with-meridians}\emojiblank & \TransparentCircle \TransparentCircle \NCDataCircle & \emojiblank \\
HelpSteer & 2023 & \cellcolor{colorCidarPropertyCounts_Datasets}{1} & \cellcolor{colorSelFeePropertyCounts_Tasks}{5} & \cellcolor{colorAgentInstructPropertyCounts_Langs}{1} & \cellcolor{colorWildChatPropertyCounts_Domains}{1} & \emoji{globe-with-meridians}\emojiblank & \CommercialDataCircle \TransparentCircle \TransparentCircle & \emojiblank \\
Pure-Dove & 2023 & \cellcolor{colorCidarPropertyCounts_Datasets}{1} & \cellcolor{colorLlama2-MedTuned-Instr.PropertyCounts_Tasks}{4} & \cellcolor{colorAgentInstructPropertyCounts_Langs}{1} & \cellcolor{colorWildChatPropertyCounts_Domains}{1} & \emojiblank\emoji{robot} & \CommercialDataCircle \TransparentCircle \TransparentCircle & \greencheck \\
Glaive Code Asst. & 2023 & \cellcolor{colorCidarPropertyCounts_Datasets}{1} & \cellcolor{colorMedicalMeadowPropertyCounts_Tasks}{2} & \cellcolor{colorCOIGPropertyCounts_Langs}{2} & \cellcolor{colorWildChatPropertyCounts_Domains}{1} & \emojiblank\emoji{robot} & \CommercialDataCircle \TransparentCircle \TransparentCircle & \emojiblank \\
No Robots & 2023 & \cellcolor{colorCidarPropertyCounts_Datasets}{1} & \cellcolor{colorCidarPropertyCounts_Tasks}{8} & \cellcolor{colorAgentInstructPropertyCounts_Langs}{1} & \cellcolor{colorWildChatPropertyCounts_Domains}{1} & \emoji{globe-with-meridians}\emojiblank & \TransparentCircle \TransparentCircle \NCDataCircle & \emojiblank \\
Open Asst. v2 & 2023 & \cellcolor{colorOpenAsst.v2PropertyCounts_Datasets}{19} & \cellcolor{colorLlama2-MedTuned-Instr.PropertyCounts_Tasks}{4} & \cellcolor{colorOpenAsst.v2PropertyCounts_Langs}{19} & \cellcolor{colorWildChatPropertyCounts_Domains}{1} & \emoji{globe-with-meridians}\emojiblank & \CommercialDataCircle \TransparentCircle \TransparentCircle & \emojiblank \\
EverythingLM & 2023 & \cellcolor{colorCidarPropertyCounts_Datasets}{1} & \cellcolor{colorCidarPropertyCounts_Tasks}{8} & \cellcolor{colorCOIGPropertyCounts_Langs}{2} & \cellcolor{colorWildChatPropertyCounts_Domains}{1} & \emojiblank\emoji{robot} & \CommercialDataCircle \TransparentCircle \TransparentCircle & \greencheck \\
UltraChat-200k & 2023 & \cellcolor{colorCidarPropertyCounts_Datasets}{1} & \cellcolor{colorWildChatPropertyCounts_Tasks}{7} & \cellcolor{colorAgentInstructPropertyCounts_Langs}{1} & \cellcolor{colorPMC-LLaMAInstr.PropertyCounts_Domains}{2} & \emojiblank\emoji{robot} & \TransparentCircle \TransparentCircle \NCDataCircle & \greencheck \\
Thai Gen AI & 2023 & \cellcolor{colorSeaBenchPropertyCounts_Datasets}{9} & \cellcolor{colorDeita10KPropertyCounts_Tasks}{11} & \cellcolor{colorAgentInstructPropertyCounts_Langs}{1} & \cellcolor{colorWildChatPropertyCounts_Domains}{1} & \emojiblank\emoji{robot} & \CommercialDataCircle \TransparentCircle \NCDataCircle & \greencheck \\
Bactrian-X & 2023 & \cellcolor{colorAgentInstructPropertyCounts_Datasets}{6} & \cellcolor{colorLlama2-MedTuned-Instr.PropertyCounts_Tasks}{4} & \cellcolor{colorBactrian-XPropertyCounts_Langs}{6} & \cellcolor{colorWildChatPropertyCounts_Domains}{1} & \emojiblank\emoji{robot} & \CommercialDataCircle \TransparentCircle \NCDataCircle & \greencheck \\
COBRA Frames & 2023 & \cellcolor{colorCidarPropertyCounts_Datasets}{1} & \cellcolor{colorPMC-LLaMAInstr.PropertyCounts_Tasks}{1} & \cellcolor{colorAgentInstructPropertyCounts_Langs}{1} & \cellcolor{colorPMC-LLaMAInstr.PropertyCounts_Domains}{2} & \emojiblank\emoji{robot} & \CommercialDataCircle \TransparentCircle \TransparentCircle & \greencheck \\
SelFee & 2023 & \cellcolor{colorCidarPropertyCounts_Datasets}{1} & \cellcolor{colorSelFeePropertyCounts_Tasks}{5} & \cellcolor{colorAgentInstructPropertyCounts_Langs}{1} & \cellcolor{colorWildChatPropertyCounts_Domains}{1} & \emojiblank\emoji{robot} & \CommercialDataCircle \TransparentCircle \TransparentCircle & \greencheck \\
Capybara & 2023 & \cellcolor{colorCapybaraPropertyCounts_Datasets}{11} & \cellcolor{colorCapybaraPropertyCounts_Tasks}{17} & \cellcolor{colorCOIGPropertyCounts_Langs}{2} & \cellcolor{colorWildChatPropertyCounts_Domains}{1} & \emojiblank\emoji{robot} & \CommercialDataCircle \UnspecifiedDataCircle \NCDataCircle & \greencheck \\
ExpertQA & 2023 & \cellcolor{colorCidarPropertyCounts_Datasets}{1} & \cellcolor{colorAgentInstructPropertyCounts_Tasks}{3} & \cellcolor{colorAgentInstructPropertyCounts_Langs}{1} & \cellcolor{colorWildChatPropertyCounts_Domains}{1} & \emojiblank\emoji{robot} & \CommercialDataCircle \TransparentCircle \TransparentCircle & \greencheck \\
ChatDoctor & 2023 & \cellcolor{colorChatDoctorPropertyCounts_Datasets}{3} & \cellcolor{colorPMC-LLaMAInstr.PropertyCounts_Tasks}{1} & \cellcolor{colorAgentInstructPropertyCounts_Langs}{1} & \cellcolor{colorPMC-LLaMAInstr.PropertyCounts_Domains}{2} & \emoji{globe-with-meridians}\emoji{robot} & \TransparentCircle \UnspecifiedDataCircle \TransparentCircle & \greencheck \\
SeaBench & 2023 & \cellcolor{colorSeaBenchPropertyCounts_Datasets}{9} & \cellcolor{colorLlama2-MedTuned-Instr.PropertyCounts_Tasks}{4} & \cellcolor{colorSeaBenchPropertyCounts_Langs}{9} & \cellcolor{colorSeaBenchPropertyCounts_Domains}{5} & \emojiblank\emoji{robot} & \CommercialDataCircle \TransparentCircle \TransparentCircle & \emojiblank \\
CollectiveCognition & 2023 & \cellcolor{colorCidarPropertyCounts_Datasets}{1} & \cellcolor{colorCollectiveCognitionPropertyCounts_Tasks}{6} & \cellcolor{colorAgentInstructPropertyCounts_Langs}{1} & \cellcolor{colorWildChatPropertyCounts_Domains}{1} & \emojiblank\emoji{robot} & \CommercialDataCircle \TransparentCircle \TransparentCircle & \greencheck \\
Deita 10K & 2023 & \cellcolor{colorWildChatPropertyCounts_Datasets}{2} & \cellcolor{colorDeita10KPropertyCounts_Tasks}{11} & \cellcolor{colorAgentInstructPropertyCounts_Langs}{1} & \cellcolor{colorDialogStudioPropertyCounts_Domains}{3} & \emojiblank\emoji{robot} & \CommercialDataCircle \TransparentCircle \NCDataCircle & \greencheck \\
PygmalionAI-PIPPA & 2023 & \cellcolor{colorCidarPropertyCounts_Datasets}{1} & \cellcolor{colorAgentInstructPropertyCounts_Tasks}{3} & \cellcolor{colorAgentInstructPropertyCounts_Langs}{1} & \cellcolor{colorWildChatPropertyCounts_Domains}{1} & \emojiblank\emoji{robot} & \CommercialDataCircle \TransparentCircle \TransparentCircle & \emojiblank \\
ChatbotArena & 2023 & \cellcolor{colorCidarPropertyCounts_Datasets}{1} & \cellcolor{colorLlama2-MedTuned-Instr.PropertyCounts_Tasks}{4} & \cellcolor{colorAgentInstructPropertyCounts_Langs}{1} & \cellcolor{colorWildChatPropertyCounts_Domains}{1} & \emojiblank\emoji{robot} & \CommercialDataCircle \TransparentCircle \NCDataCircle & \greencheck \\
OpenMathInstr.-1 & 2024 & \cellcolor{colorWildChatPropertyCounts_Datasets}{2} & \cellcolor{colorAgentInstructPropertyCounts_Tasks}{3} & \cellcolor{colorAgentInstructPropertyCounts_Langs}{1} & \cellcolor{colorDialogStudioPropertyCounts_Domains}{3} & \emojiblank\emoji{robot} & \CommercialDataCircle \UnspecifiedDataCircle \TransparentCircle & \emojiblank \\
Orca-Math & 2024 & \cellcolor{colorCidarPropertyCounts_Datasets}{1} & \cellcolor{colorPMC-LLaMAInstr.PropertyCounts_Tasks}{1} & \cellcolor{colorAgentInstructPropertyCounts_Langs}{1} & \cellcolor{colorDialogStudioPropertyCounts_Domains}{3} & \emojiblank\emoji{robot} & \CommercialDataCircle \TransparentCircle \NCDataCircle & \greencheck \\
10k Prompt Ranked & 2024 & \cellcolor{colorCidarPropertyCounts_Datasets}{1} & \cellcolor{colorCOIGPropertyCounts_Tasks}{13} & \cellcolor{colorAgentInstructPropertyCounts_Langs}{1} & \cellcolor{color10kPromptRankedPropertyCounts_Domains}{4} & \emojiblank\emoji{robot} & \TransparentCircle \UnspecifiedDataCircle \TransparentCircle & \greencheck \\
LongAlign-10k & 2024 & \cellcolor{colorCidarPropertyCounts_Datasets}{1} & \cellcolor{colorAgentInstructPropertyCounts_Tasks}{3} & \cellcolor{colorAgentInstructPropertyCounts_Langs}{1} & \cellcolor{colorWildChatPropertyCounts_Domains}{1} & \emojiblank\emoji{robot} & \CommercialDataCircle \TransparentCircle \NCDataCircle & \greencheck \\
Llama2-MedTuned-Instr. & 2024 & \cellcolor{colorCidarPropertyCounts_Datasets}{1} & \cellcolor{colorLlama2-MedTuned-Instr.PropertyCounts_Tasks}{4} & \cellcolor{colorAgentInstructPropertyCounts_Langs}{1} & \cellcolor{colorWildChatPropertyCounts_Domains}{1} & \emoji{globe-with-meridians}\emojiblank & \TransparentCircle \TransparentCircle \NCDataCircle & \emojiblank \\
KIWI & 2024 & \cellcolor{colorCidarPropertyCounts_Datasets}{1} & \cellcolor{colorPMC-LLaMAInstr.PropertyCounts_Tasks}{1} & \cellcolor{colorAgentInstructPropertyCounts_Langs}{1} & \cellcolor{colorPMC-LLaMAInstr.PropertyCounts_Domains}{2} & \emojiblank\emoji{robot} & \CommercialDataCircle \TransparentCircle \TransparentCircle & \greencheck \\
Indic-Instr. & 2024 & \cellcolor{colorMedicalMeadowPropertyCounts_Datasets}{8} & \cellcolor{colorWildChatPropertyCounts_Tasks}{7} & \cellcolor{colorCOIGPropertyCounts_Langs}{2} & \cellcolor{colorDialogStudioPropertyCounts_Domains}{3} & \emojiblank\emoji{robot} & \CommercialDataCircle \UnspecifiedDataCircle \NCDataCircle & \greencheck \\
Gretel Text-to-SQL & 2024 & \cellcolor{colorCidarPropertyCounts_Datasets}{1} & \cellcolor{colorPMC-LLaMAInstr.PropertyCounts_Tasks}{1} & \cellcolor{colorGretelText-to-SQLPropertyCounts_Langs}{3} & \cellcolor{colorWildChatPropertyCounts_Domains}{1} & \emojiblank\emoji{robot} & \CommercialDataCircle \TransparentCircle \TransparentCircle & \emojiblank \\
Conifer & 2024 & \cellcolor{colorCidarPropertyCounts_Datasets}{1} & \cellcolor{colorCidarPropertyCounts_Tasks}{8} & \cellcolor{colorAgentInstructPropertyCounts_Langs}{1} & \cellcolor{colorPMC-LLaMAInstr.PropertyCounts_Domains}{2} & \emojiblank\emoji{robot} & \CommercialDataCircle \TransparentCircle \TransparentCircle & \greencheck \\
Cidar & 2024 & \cellcolor{colorCidarPropertyCounts_Datasets}{1} & \cellcolor{colorCidarPropertyCounts_Tasks}{8} & \cellcolor{colorAgentInstructPropertyCounts_Langs}{1} & \cellcolor{colorWildChatPropertyCounts_Domains}{1} & \emojiblank\emoji{robot} & \TransparentCircle \TransparentCircle \NCDataCircle & \greencheck \\
Aya & 2024 & \cellcolor{colorAyaPropertyCounts_Datasets}{71} & \cellcolor{colorWildChatPropertyCounts_Tasks}{7} & \cellcolor{colorAyaPropertyCounts_Langs}{71} & \cellcolor{colorWildChatPropertyCounts_Domains}{1} & \emoji{globe-with-meridians}\emojiblank & \CommercialDataCircle \TransparentCircle \TransparentCircle & \emojiblank \\
WildChat & 2024 & \cellcolor{colorWildChatPropertyCounts_Datasets}{2} & \cellcolor{colorWildChatPropertyCounts_Tasks}{7} & \cellcolor{colorWildChatPropertyCounts_Langs}{10} & \cellcolor{colorWildChatPropertyCounts_Domains}{1} & \emojiblank\emoji{robot} & \CommercialDataCircle \TransparentCircle \TransparentCircle & \greencheck \\
Medical Meadow & Mult. & \cellcolor{colorMedicalMeadowPropertyCounts_Datasets}{8} & \cellcolor{colorMedicalMeadowPropertyCounts_Tasks}{2} & \cellcolor{colorAgentInstructPropertyCounts_Langs}{1} & \cellcolor{colorDialogStudioPropertyCounts_Domains}{3} & \emoji{globe-with-meridians}\emoji{robot} & \CommercialDataCircle \UnspecifiedDataCircle \NCDataCircle & \greencheck \\
PMC-LLaMA Instr. & Mult. & \cellcolor{colorPMC-LLaMAInstr.PropertyCounts_Datasets}{7} & \cellcolor{colorPMC-LLaMAInstr.PropertyCounts_Tasks}{1} & \cellcolor{colorAgentInstructPropertyCounts_Langs}{1} & \cellcolor{colorPMC-LLaMAInstr.PropertyCounts_Domains}{2} & \emoji{globe-with-meridians}\emoji{robot} & \CommercialDataCircle \UnspecifiedDataCircle \TransparentCircle & \greencheck \\
DialogStudio & Mult. & \cellcolor{colorDialogStudioPropertyCounts_Datasets}{83} & \cellcolor{colorAgentInstructPropertyCounts_Tasks}{3} & \cellcolor{colorDialogStudioPropertyCounts_Langs}{5} & \cellcolor{colorDialogStudioPropertyCounts_Domains}{3} & \emoji{globe-with-meridians}\emoji{robot} & \CommercialDataCircle \UnspecifiedDataCircle \NCDataCircle & \emojiblank \\
COIG & Mult. & \cellcolor{colorCOIGPropertyCounts_Datasets}{18} & \cellcolor{colorCOIGPropertyCounts_Tasks}{13} & \cellcolor{colorCOIGPropertyCounts_Langs}{2} & \cellcolor{colorCOIGPropertyCounts_Domains}{22} & \emoji{globe-with-meridians}\emoji{robot} & \CommercialDataCircle \UnspecifiedDataCircle \NCDataCircle & \emojiblank \\
AgentInstruct & Mult. & \cellcolor{colorAgentInstructPropertyCounts_Datasets}{6} & \cellcolor{colorAgentInstructPropertyCounts_Tasks}{3} & \cellcolor{colorAgentInstructPropertyCounts_Langs}{1} & \cellcolor{colorAgentInstructPropertyCounts_Domains}{7} & \emoji{globe-with-meridians}\emoji{robot} & \CommercialDataCircle \UnspecifiedDataCircle \TransparentCircle & \greencheck \\
Open-Platypus & Mult. & \cellcolor{colorOpen-PlatypusPropertyCounts_Datasets}{10} & \cellcolor{colorOpen-PlatypusPropertyCounts_Tasks}{10} & \cellcolor{colorOpen-PlatypusPropertyCounts_Langs}{36} & \cellcolor{colorOpen-PlatypusPropertyCounts_Domains}{8} & \emoji{globe-with-meridians}\emoji{robot} & \CommercialDataCircle \UnspecifiedDataCircle \NCDataCircle & \greencheck \\
\end{longtable}
\setlength{\tabcolsep}{1.9pt}
\definecolor{colorTIMITPropertyCounts_Hr}{RGB}{244,229,189}
\definecolor{colorSwitchboardPropertyCounts_Hr}{RGB}{245,241,232}
\definecolor{colorAfricanAcc.FrenchPropertyCounts_Hr}{RGB}{245,235,206}
\definecolor{colorCSJPropertyCounts_Hr}{RGB}{245,244,242}
\definecolor{colorFisherPropertyCounts_Hr}{RGB}{236,243,242}
\definecolor{colorCSLU22Langs.PropertyCounts_Hr}{RGB}{245,238,220}
\definecolor{colorAMIPropertyCounts_Hr}{RGB}{245,239,222}
\definecolor{colorCSLU1.2PropertyCounts_Hr}{RGB}{245,235,208}
\definecolor{colorALLSSTARPropertyCounts_Hr}{RGB}{245,238,220}
\definecolor{colorTED-LIUM3PropertyCounts_Hr}{RGB}{245,243,238}
\definecolor{colorNSTNorwegianPropertyCounts_Hr}{RGB}{245,243,240}
\definecolor{colorNSTDanishPropertyCounts_Hr}{RGB}{245,243,240}
\definecolor{colorNSTSwedishPropertyCounts_Hr}{RGB}{245,242,234}
\definecolor{colorVystadialPropertyCounts_Hr}{RGB}{245,237,216}
\definecolor{colorTHCHS-30PropertyCounts_Hr}{RGB}{245,236,212}
\definecolor{colorLibriSpeechPropertyCounts_Hr}{RGB}{244,244,244}
\definecolor{colorTHUYG-20PropertyCounts_Hr}{RGB}{245,235,206}
\definecolor{colorVCTKPropertyCounts_Hr}{RGB}{245,237,214}
\definecolor{colorSpokenWikipediaPropertyCounts_Hr}{RGB}{244,244,244}
\definecolor{colorAISHELL-1PropertyCounts_Hr}{RGB}{245,243,240}
\definecolor{colorLJSpeechPropertyCounts_Hr}{RGB}{245,235,208}
\definecolor{colorClarinPLPropertyCounts_Hr}{RGB}{245,237,216}
\definecolor{colorAISHELL-2PropertyCounts_Hr}{RGB}{244,244,244}
\definecolor{colorRegionalAf.Am.Lang.PropertyCounts_Hr}{RGB}{245,240,228}
\definecolor{colorCrowdSourcedSpeechPropertyCounts_Hr}{RGB}{242,244,244}
\definecolor{colorZeroth-KoreanPropertyCounts_Hr}{RGB}{245,239,222}
\definecolor{colorRTVEPropertyCounts_Hr}{RGB}{245,244,242}
\definecolor{colorOpenSTTPropertyCounts_Hr}{RGB}{215,237,234}
\definecolor{colorMuST-CPropertyCounts_Hr}{RGB}{231,241,240}
\definecolor{colorM-AILABSPropertyCounts_Hr}{RGB}{244,244,244}
\definecolor{colorMAGICDATAPropertyCounts_Hr}{RGB}{245,244,244}
\definecolor{colorCommonVoice17PropertyCounts_Hr}{RGB}{211,237,233}
\definecolor{colorCoNASEPropertyCounts_Hr}{RGB}{193,231,226}
\definecolor{colorNigerianEnglishPropertyCounts_Hr}{RGB}{245,230,192}
\definecolor{colorNorwegianParl.SpeechPropertyCounts_Hr}{RGB}{245,240,226}
\definecolor{color120hSpanishSpeechPropertyCounts_Hr}{RGB}{245,239,224}
\definecolor{colorDiDiSpeechPropertyCounts_Hr}{RGB}{245,244,244}
\definecolor{colorCzechParliamentPropertyCounts_Hr}{RGB}{245,243,238}
\definecolor{colorCoVoST-2PropertyCounts_Hr}{RGB}{233,242,240}
\definecolor{colorKSCPropertyCounts_Hr}{RGB}{245,242,234}
\definecolor{colorBasq.,Cat.andGal.PropertyCounts_Hr}{RGB}{245,236,210}
\definecolor{colorKsponSpeechPropertyCounts_Hr}{RGB}{244,244,244}
\definecolor{colorSamromurPropertyCounts_Hr}{RGB}{245,240,226}
\definecolor{colorMultiling.LibriSpeechPropertyCounts_Hr}{RGB}{206,235,231}
\definecolor{colorMaSSPropertyCounts_Hr}{RGB}{245,240,228}
\definecolor{colorFTSPEECHPropertyCounts_Hr}{RGB}{236,243,242}
\definecolor{colorEng.Acc.inBrit.IslesPropertyCounts_Hr}{RGB}{245,236,210}
\definecolor{colorHighlandPueblaNahuatlPropertyCounts_Hr}{RGB}{245,240,226}
\definecolor{colorQASRPropertyCounts_Hr}{RGB}{236,243,242}
\definecolor{colorMultiling.TEDxPropertyCounts_Hr}{RGB}{245,244,244}
\definecolor{colorMinds14PropertyCounts_Hr}{RGB}{245,235,208}
\definecolor{colorGolosPropertyCounts_Hr}{RGB}{242,244,244}
\definecolor{colorMASCPropertyCounts_Hr}{RGB}{242,244,244}
\definecolor{colorLaboroTVSpeechPropertyCounts_Hr}{RGB}{236,243,242}
\definecolor{colorKeSpeechPropertyCounts_Hr}{RGB}{238,243,242}
\definecolor{colorJTUBESPEECHPropertyCounts_Hr}{RGB}{240,243,243}
\definecolor{colorGigaSpeechPropertyCounts_Hr}{RGB}{222,239,237}
\definecolor{colorVoxPopuliPropertyCounts_Hr}{RGB}{238,243,242}
\definecolor{colorSPGISpeechPropertyCounts_Hr}{RGB}{227,240,239}
\definecolor{colorWestAfr.RadioPropertyCounts_Hr}{RGB}{245,240,226}
\definecolor{colorAISHELL-4PropertyCounts_Hr}{RGB}{245,239,224}
\definecolor{colorWestAfr.Virt.Asst.PropertyCounts_Hr}{RGB}{239,221,175}
\definecolor{colorMediaSpeechPropertyCounts_Hr}{RGB}{245,236,212}
\definecolor{colorPeople'sSpeechPropertyCounts_Hr}{RGB}{211,237,233}
\definecolor{color1111HoursHindiPropertyCounts_Hr}{RGB}{245,239,224}
\definecolor{colorShrutilipiPropertyCounts_Hr}{RGB}{226,240,238}
\definecolor{colorWenetSpeechPropertyCounts_Hr}{RGB}{222,239,237}
\definecolor{colorSamromurChildrenPropertyCounts_Hr}{RGB}{245,240,226}
\definecolor{colorSDS-200PropertyCounts_Hr}{RGB}{245,241,230}
\definecolor{coloraidatatangPropertyCounts_Hr}{RGB}{245,241,230}
\definecolor{colorFleursPropertyCounts_Hr}{RGB}{240,243,243}
\definecolor{colorOLKAVSPropertyCounts_Hr}{RGB}{242,244,244}
\definecolor{colorNorwegianParl.PropertyCounts_Hr}{RGB}{245,240,226}
\definecolor{colorMagicData-RAMCPropertyCounts_Hr}{RGB}{245,240,228}
\definecolor{colorKathbathPropertyCounts_Hr}{RGB}{238,243,242}
\definecolor{colorHebrewKanPropertyCounts_Hr}{RGB}{245,232,196}
\definecolor{colorHebrewCourseraPropertyCounts_Hr}{RGB}{245,236,212}
\definecolor{colorBloomSpeechPropertyCounts_Hr}{RGB}{245,243,238}
\definecolor{colorEnglish-VietnamesePropertyCounts_Hr}{RGB}{245,243,240}
\definecolor{colorEarnings-22PropertyCounts_Hr}{RGB}{245,239,224}
\definecolor{colorYODASPropertyCounts_Hr}{RGB}{179,226,219}
\definecolor{colorAFRISPEECH-200PropertyCounts_Hr}{RGB}{245,241,230}
\definecolor{colorAaltoFinnishParl.PropertyCounts_Hr}{RGB}{233,242,240}
\definecolor{colorReazonSpeechPropertyCounts_Hr}{RGB}{209,236,232}
\definecolor{colorEdAccPropertyCounts_Hr}{RGB}{245,236,212}
\definecolor{colorRixVoxPropertyCounts_Hr}{RGB}{227,240,239}
\definecolor{colorJapaneseAnimeSpeechPropertyCounts_Hr}{RGB}{245,239,224}
\definecolor{colorSnowMountainPropertyCounts_Hr}{RGB}{245,241,232}
\definecolor{colorSamromurMilljonPropertyCounts_Hr}{RGB}{244,244,244}
\definecolor{colorBud500PropertyCounts_Hr}{RGB}{245,243,240}
\definecolor{colorVibraVoxPropertyCounts_Hr}{RGB}{245,234,204}
\definecolor{colorM2ASRPropertyCounts_Hr}{RGB}{245,243,238}
\definecolor{colorTIMITPropertyCounts_Spkr}{RGB}{215,237,234}
\definecolor{colorSwitchboardPropertyCounts_Spkr}{RGB}{215,237,234}
\definecolor{colorAfricanAcc.FrenchPropertyCounts_Spkr}{RGB}{218,238,235}
\definecolor{colorCSJPropertyCounts_Spkr}{RGB}{211,237,233}
\definecolor{colorFisherPropertyCounts_Spkr}{RGB}{202,234,230}
\definecolor{colorCSLU22Langs.PropertyCounts_Spkr}{RGB}{240,223,178}
\definecolor{colorAMIPropertyCounts_Spkr}{RGB}{240,223,178}
\definecolor{colorCSLU1.2PropertyCounts_Spkr}{RGB}{206,235,231}
\definecolor{colorALLSSTARPropertyCounts_Spkr}{RGB}{220,239,236}
\definecolor{colorTED-LIUM3PropertyCounts_Spkr}{RGB}{209,236,232}
\definecolor{colorNSTNorwegianPropertyCounts_Spkr}{RGB}{213,237,234}
\definecolor{colorNSTDanishPropertyCounts_Spkr}{RGB}{240,223,178}
\definecolor{colorNSTSwedishPropertyCounts_Spkr}{RGB}{240,223,178}
\definecolor{colorVystadialPropertyCounts_Spkr}{RGB}{240,223,178}
\definecolor{colorTHCHS-30PropertyCounts_Spkr}{RGB}{226,240,238}
\definecolor{colorLibriSpeechPropertyCounts_Spkr}{RGB}{208,236,232}
\definecolor{colorTHUYG-20PropertyCounts_Spkr}{RGB}{217,238,235}
\definecolor{colorVCTKPropertyCounts_Spkr}{RGB}{222,239,237}
\definecolor{colorSpokenWikipediaPropertyCounts_Spkr}{RGB}{213,237,234}
\definecolor{colorAISHELL-1PropertyCounts_Spkr}{RGB}{217,238,235}
\definecolor{colorLJSpeechPropertyCounts_Spkr}{RGB}{242,244,244}
\definecolor{colorClarinPLPropertyCounts_Spkr}{RGB}{217,238,235}
\definecolor{colorAISHELL-2PropertyCounts_Spkr}{RGB}{209,236,232}
\definecolor{colorRegionalAf.Am.Lang.PropertyCounts_Spkr}{RGB}{218,238,235}
\definecolor{colorCrowdSourcedSpeechPropertyCounts_Spkr}{RGB}{208,236,232}
\definecolor{colorZeroth-KoreanPropertyCounts_Spkr}{RGB}{220,239,236}
\definecolor{colorRTVEPropertyCounts_Spkr}{RGB}{240,223,178}
\definecolor{colorOpenSTTPropertyCounts_Spkr}{RGB}{240,223,178}
\definecolor{colorMuST-CPropertyCounts_Spkr}{RGB}{209,236,232}
\definecolor{colorM-AILABSPropertyCounts_Spkr}{RGB}{240,223,178}
\definecolor{colorMAGICDATAPropertyCounts_Spkr}{RGB}{211,237,233}
\definecolor{colorCommonVoice17PropertyCounts_Spkr}{RGB}{179,226,219}
\definecolor{colorCoNASEPropertyCounts_Spkr}{RGB}{240,223,178}
\definecolor{colorNigerianEnglishPropertyCounts_Spkr}{RGB}{240,223,178}
\definecolor{colorNorwegianParl.SpeechPropertyCounts_Spkr}{RGB}{217,238,235}
\definecolor{color120hSpanishSpeechPropertyCounts_Spkr}{RGB}{229,241,239}
\definecolor{colorDiDiSpeechPropertyCounts_Spkr}{RGB}{204,235,230}
\definecolor{colorCzechParliamentPropertyCounts_Spkr}{RGB}{218,238,235}
\definecolor{colorCoVoST-2PropertyCounts_Spkr}{RGB}{190,230,224}
\definecolor{colorKSCPropertyCounts_Spkr}{RGB}{240,223,178}
\definecolor{colorBasq.,Cat.andGal.PropertyCounts_Spkr}{RGB}{220,239,236}
\definecolor{colorKsponSpeechPropertyCounts_Spkr}{RGB}{209,236,232}
\definecolor{colorSamromurPropertyCounts_Spkr}{RGB}{202,234,230}
\definecolor{colorMultiling.LibriSpeechPropertyCounts_Spkr}{RGB}{204,235,230}
\definecolor{colorMaSSPropertyCounts_Spkr}{RGB}{240,223,178}
\definecolor{colorFTSPEECHPropertyCounts_Spkr}{RGB}{217,238,235}
\definecolor{colorEng.Acc.inBrit.IslesPropertyCounts_Spkr}{RGB}{222,239,237}
\definecolor{colorHighlandPueblaNahuatlPropertyCounts_Spkr}{RGB}{240,223,178}
\definecolor{colorQASRPropertyCounts_Spkr}{RGB}{202,234,230}
\definecolor{colorMultiling.TEDxPropertyCounts_Spkr}{RGB}{240,223,178}
\definecolor{colorMinds14PropertyCounts_Spkr}{RGB}{240,223,178}
\definecolor{colorGolosPropertyCounts_Spkr}{RGB}{240,223,178}
\definecolor{colorMASCPropertyCounts_Spkr}{RGB}{200,234,229}
\definecolor{colorLaboroTVSpeechPropertyCounts_Spkr}{RGB}{240,223,178}
\definecolor{colorKeSpeechPropertyCounts_Spkr}{RGB}{199,234,229}
\definecolor{colorJTUBESPEECHPropertyCounts_Spkr}{RGB}{240,223,178}
\definecolor{colorGigaSpeechPropertyCounts_Spkr}{RGB}{240,223,178}
\definecolor{colorVoxPopuliPropertyCounts_Spkr}{RGB}{206,235,231}
\definecolor{colorSPGISpeechPropertyCounts_Spkr}{RGB}{193,231,226}
\definecolor{colorWestAfr.RadioPropertyCounts_Spkr}{RGB}{240,223,178}
\definecolor{colorAISHELL-4PropertyCounts_Spkr}{RGB}{224,240,237}
\definecolor{colorWestAfr.Virt.Asst.PropertyCounts_Spkr}{RGB}{226,240,238}
\definecolor{colorMediaSpeechPropertyCounts_Spkr}{RGB}{240,223,178}
\definecolor{colorPeople'sSpeechPropertyCounts_Spkr}{RGB}{240,223,178}
\definecolor{color1111HoursHindiPropertyCounts_Spkr}{RGB}{240,223,178}
\definecolor{colorShrutilipiPropertyCounts_Spkr}{RGB}{240,223,178}
\definecolor{colorWenetSpeechPropertyCounts_Spkr}{RGB}{240,223,178}
\definecolor{colorSamromurChildrenPropertyCounts_Spkr}{RGB}{208,236,232}
\definecolor{colorSDS-200PropertyCounts_Spkr}{RGB}{206,235,231}
\definecolor{coloraidatatangPropertyCounts_Spkr}{RGB}{215,237,234}
\definecolor{colorFleursPropertyCounts_Spkr}{RGB}{240,223,178}
\definecolor{colorOLKAVSPropertyCounts_Spkr}{RGB}{211,237,233}
\definecolor{colorNorwegianParl.PropertyCounts_Spkr}{RGB}{218,238,235}
\definecolor{colorMagicData-RAMCPropertyCounts_Spkr}{RGB}{213,237,234}
\definecolor{colorKathbathPropertyCounts_Spkr}{RGB}{211,237,233}
\definecolor{colorHebrewKanPropertyCounts_Spkr}{RGB}{240,223,178}
\definecolor{colorHebrewCourseraPropertyCounts_Spkr}{RGB}{240,223,178}
\definecolor{colorBloomSpeechPropertyCounts_Spkr}{RGB}{240,223,178}
\definecolor{colorEnglish-VietnamesePropertyCounts_Spkr}{RGB}{240,223,178}
\definecolor{colorEarnings-22PropertyCounts_Spkr}{RGB}{222,239,237}
\definecolor{colorYODASPropertyCounts_Spkr}{RGB}{240,223,178}
\definecolor{colorAFRISPEECH-200PropertyCounts_Spkr}{RGB}{208,236,232}
\definecolor{colorAaltoFinnishParl.PropertyCounts_Spkr}{RGB}{215,237,234}
\definecolor{colorReazonSpeechPropertyCounts_Spkr}{RGB}{240,223,178}
\definecolor{colorEdAccPropertyCounts_Spkr}{RGB}{222,239,237}
\definecolor{colorRixVoxPropertyCounts_Spkr}{RGB}{240,223,178}
\definecolor{colorJapaneseAnimeSpeechPropertyCounts_Spkr}{RGB}{240,223,178}
\definecolor{colorSnowMountainPropertyCounts_Spkr}{RGB}{231,241,240}
\definecolor{colorSamromurMilljonPropertyCounts_Spkr}{RGB}{200,234,229}
\definecolor{colorBud500PropertyCounts_Spkr}{RGB}{240,223,178}
\definecolor{colorVibraVoxPropertyCounts_Spkr}{RGB}{218,238,235}
\definecolor{colorM2ASRPropertyCounts_Spkr}{RGB}{215,237,234}
\definecolor{colorTIMITPropertyCounts_Lang}{RGB}{240,223,178}
\definecolor{colorSwitchboardPropertyCounts_Lang}{RGB}{240,223,178}
\definecolor{colorAfricanAcc.FrenchPropertyCounts_Lang}{RGB}{240,223,178}
\definecolor{colorCSJPropertyCounts_Lang}{RGB}{240,223,178}
\definecolor{colorFisherPropertyCounts_Lang}{RGB}{240,223,178}
\definecolor{colorCSLU22Langs.PropertyCounts_Lang}{RGB}{233,242,240}
\definecolor{colorAMIPropertyCounts_Lang}{RGB}{240,223,178}
\definecolor{colorCSLU1.2PropertyCounts_Lang}{RGB}{240,223,178}
\definecolor{colorALLSSTARPropertyCounts_Lang}{RGB}{226,240,238}
\definecolor{colorTED-LIUM3PropertyCounts_Lang}{RGB}{240,223,178}
\definecolor{colorNSTNorwegianPropertyCounts_Lang}{RGB}{240,223,178}
\definecolor{colorNSTDanishPropertyCounts_Lang}{RGB}{240,223,178}
\definecolor{colorNSTSwedishPropertyCounts_Lang}{RGB}{240,223,178}
\definecolor{colorVystadialPropertyCounts_Lang}{RGB}{245,233,198}
\definecolor{colorTHCHS-30PropertyCounts_Lang}{RGB}{240,223,178}
\definecolor{colorLibriSpeechPropertyCounts_Lang}{RGB}{240,223,178}
\definecolor{colorTHUYG-20PropertyCounts_Lang}{RGB}{240,223,178}
\definecolor{colorVCTKPropertyCounts_Lang}{RGB}{240,223,178}
\definecolor{colorSpokenWikipediaPropertyCounts_Lang}{RGB}{245,236,210}
\definecolor{colorAISHELL-1PropertyCounts_Lang}{RGB}{240,223,178}
\definecolor{colorLJSpeechPropertyCounts_Lang}{RGB}{240,223,178}
\definecolor{colorClarinPLPropertyCounts_Lang}{RGB}{240,223,178}
\definecolor{colorAISHELL-2PropertyCounts_Lang}{RGB}{240,223,178}
\definecolor{colorRegionalAf.Am.Lang.PropertyCounts_Lang}{RGB}{240,223,178}
\definecolor{colorCrowdSourcedSpeechPropertyCounts_Lang}{RGB}{245,239,222}
\definecolor{colorZeroth-KoreanPropertyCounts_Lang}{RGB}{240,223,178}
\definecolor{colorRTVEPropertyCounts_Lang}{RGB}{240,223,178}
\definecolor{colorOpenSTTPropertyCounts_Lang}{RGB}{240,223,178}
\definecolor{colorMuST-CPropertyCounts_Lang}{RGB}{238,243,242}
\definecolor{colorM-AILABSPropertyCounts_Lang}{RGB}{245,242,234}
\definecolor{colorMAGICDATAPropertyCounts_Lang}{RGB}{240,223,178}
\definecolor{colorCommonVoice17PropertyCounts_Lang}{RGB}{187,229,223}
\definecolor{colorCoNASEPropertyCounts_Lang}{RGB}{240,223,178}
\definecolor{colorNigerianEnglishPropertyCounts_Lang}{RGB}{240,223,178}
\definecolor{colorNorwegianParl.SpeechPropertyCounts_Lang}{RGB}{240,223,178}
\definecolor{color120hSpanishSpeechPropertyCounts_Lang}{RGB}{240,223,178}
\definecolor{colorDiDiSpeechPropertyCounts_Lang}{RGB}{240,223,178}
\definecolor{colorCzechParliamentPropertyCounts_Lang}{RGB}{240,223,178}
\definecolor{colorCoVoST-2PropertyCounts_Lang}{RGB}{231,241,240}
\definecolor{colorKSCPropertyCounts_Lang}{RGB}{240,223,178}
\definecolor{colorBasq.,Cat.andGal.PropertyCounts_Lang}{RGB}{245,236,210}
\definecolor{colorKsponSpeechPropertyCounts_Lang}{RGB}{240,223,178}
\definecolor{colorSamromurPropertyCounts_Lang}{RGB}{240,223,178}
\definecolor{colorMultiling.LibriSpeechPropertyCounts_Lang}{RGB}{245,242,234}
\definecolor{colorMaSSPropertyCounts_Lang}{RGB}{245,242,234}
\definecolor{colorFTSPEECHPropertyCounts_Lang}{RGB}{240,223,178}
\definecolor{colorEng.Acc.inBrit.IslesPropertyCounts_Lang}{RGB}{240,223,178}
\definecolor{colorHighlandPueblaNahuatlPropertyCounts_Lang}{RGB}{240,223,178}
\definecolor{colorQASRPropertyCounts_Lang}{RGB}{240,223,178}
\definecolor{colorMultiling.TEDxPropertyCounts_Lang}{RGB}{245,243,238}
\definecolor{colorMinds14PropertyCounts_Lang}{RGB}{242,244,244}
\definecolor{colorGolosPropertyCounts_Lang}{RGB}{240,223,178}
\definecolor{colorMASCPropertyCounts_Lang}{RGB}{240,223,178}
\definecolor{colorLaboroTVSpeechPropertyCounts_Lang}{RGB}{245,233,198}
\definecolor{colorKeSpeechPropertyCounts_Lang}{RGB}{245,233,198}
\definecolor{colorJTUBESPEECHPropertyCounts_Lang}{RGB}{245,233,198}
\definecolor{colorGigaSpeechPropertyCounts_Lang}{RGB}{240,223,178}
\definecolor{colorVoxPopuliPropertyCounts_Lang}{RGB}{238,243,242}
\definecolor{colorSPGISpeechPropertyCounts_Lang}{RGB}{240,223,178}
\definecolor{colorWestAfr.RadioPropertyCounts_Lang}{RGB}{245,243,240}
\definecolor{colorAISHELL-4PropertyCounts_Lang}{RGB}{240,223,178}
\definecolor{colorWestAfr.Virt.Asst.PropertyCounts_Lang}{RGB}{245,236,210}
\definecolor{colorMediaSpeechPropertyCounts_Lang}{RGB}{245,237,216}
\definecolor{colorPeople'sSpeechPropertyCounts_Lang}{RGB}{240,223,178}
\definecolor{color1111HoursHindiPropertyCounts_Lang}{RGB}{240,223,178}
\definecolor{colorShrutilipiPropertyCounts_Lang}{RGB}{245,244,244}
\definecolor{colorWenetSpeechPropertyCounts_Lang}{RGB}{240,223,178}
\definecolor{colorSamromurChildrenPropertyCounts_Lang}{RGB}{240,223,178}
\definecolor{colorSDS-200PropertyCounts_Lang}{RGB}{240,223,178}
\definecolor{coloraidatatangPropertyCounts_Lang}{RGB}{240,223,178}
\definecolor{colorFleursPropertyCounts_Lang}{RGB}{193,231,226}
\definecolor{colorOLKAVSPropertyCounts_Lang}{RGB}{240,223,178}
\definecolor{colorNorwegianParl.PropertyCounts_Lang}{RGB}{240,223,178}
\definecolor{colorMagicData-RAMCPropertyCounts_Lang}{RGB}{240,223,178}
\definecolor{colorKathbathPropertyCounts_Lang}{RGB}{245,244,244}
\definecolor{colorHebrewKanPropertyCounts_Lang}{RGB}{240,223,178}
\definecolor{colorHebrewCourseraPropertyCounts_Lang}{RGB}{240,223,178}
\definecolor{colorBloomSpeechPropertyCounts_Lang}{RGB}{209,236,232}
\definecolor{colorEnglish-VietnamesePropertyCounts_Lang}{RGB}{245,233,198}
\definecolor{colorEarnings-22PropertyCounts_Lang}{RGB}{240,223,178}
\definecolor{colorYODASPropertyCounts_Lang}{RGB}{179,226,219}
\definecolor{colorAFRISPEECH-200PropertyCounts_Lang}{RGB}{233,242,240}
\definecolor{colorAaltoFinnishParl.PropertyCounts_Lang}{RGB}{240,223,178}
\definecolor{colorReazonSpeechPropertyCounts_Lang}{RGB}{240,223,178}
\definecolor{colorEdAccPropertyCounts_Lang}{RGB}{240,223,178}
\definecolor{colorRixVoxPropertyCounts_Lang}{RGB}{240,223,178}
\definecolor{colorJapaneseAnimeSpeechPropertyCounts_Lang}{RGB}{240,223,178}
\definecolor{colorSnowMountainPropertyCounts_Lang}{RGB}{242,244,244}
\definecolor{colorSamromurMilljonPropertyCounts_Lang}{RGB}{240,223,178}
\definecolor{colorBud500PropertyCounts_Lang}{RGB}{240,223,178}
\definecolor{colorVibraVoxPropertyCounts_Lang}{RGB}{240,223,178}
\definecolor{colorM2ASRPropertyCounts_Lang}{RGB}{245,237,216}
\definecolor{colorTIMITPropertyCounts_Creat}{RGB}{245,242,234}
\definecolor{colorSwitchboardPropertyCounts_Creat}{RGB}{240,223,178}
\definecolor{colorAfricanAcc.FrenchPropertyCounts_Creat}{RGB}{240,223,178}
\definecolor{colorCSJPropertyCounts_Creat}{RGB}{240,223,178}
\definecolor{colorFisherPropertyCounts_Creat}{RGB}{240,223,178}
\definecolor{colorCSLU22Langs.PropertyCounts_Creat}{RGB}{240,223,178}
\definecolor{colorAMIPropertyCounts_Creat}{RGB}{240,223,178}
\definecolor{colorCSLU1.2PropertyCounts_Creat}{RGB}{240,223,178}
\definecolor{colorALLSSTARPropertyCounts_Creat}{RGB}{240,223,178}
\definecolor{colorTED-LIUM3PropertyCounts_Creat}{RGB}{245,237,214}
\definecolor{colorNSTNorwegianPropertyCounts_Creat}{RGB}{240,223,178}
\definecolor{colorNSTDanishPropertyCounts_Creat}{RGB}{240,223,178}
\definecolor{colorNSTSwedishPropertyCounts_Creat}{RGB}{240,223,178}
\definecolor{colorVystadialPropertyCounts_Creat}{RGB}{240,223,178}
\definecolor{colorTHCHS-30PropertyCounts_Creat}{RGB}{240,223,178}
\definecolor{colorLibriSpeechPropertyCounts_Creat}{RGB}{240,223,178}
\definecolor{colorTHUYG-20PropertyCounts_Creat}{RGB}{245,237,214}
\definecolor{colorVCTKPropertyCounts_Creat}{RGB}{240,223,178}
\definecolor{colorSpokenWikipediaPropertyCounts_Creat}{RGB}{240,223,178}
\definecolor{colorAISHELL-1PropertyCounts_Creat}{RGB}{245,237,214}
\definecolor{colorLJSpeechPropertyCounts_Creat}{RGB}{240,223,178}
\definecolor{colorClarinPLPropertyCounts_Creat}{RGB}{240,223,178}
\definecolor{colorAISHELL-2PropertyCounts_Creat}{RGB}{245,237,214}
\definecolor{colorRegionalAf.Am.Lang.PropertyCounts_Creat}{RGB}{240,223,178}
\definecolor{colorCrowdSourcedSpeechPropertyCounts_Creat}{RGB}{240,223,178}
\definecolor{colorZeroth-KoreanPropertyCounts_Creat}{RGB}{240,223,178}
\definecolor{colorRTVEPropertyCounts_Creat}{RGB}{240,223,178}
\definecolor{colorOpenSTTPropertyCounts_Creat}{RGB}{245,237,214}
\definecolor{colorMuST-CPropertyCounts_Creat}{RGB}{245,237,214}
\definecolor{colorM-AILABSPropertyCounts_Creat}{RGB}{240,223,178}
\definecolor{colorMAGICDATAPropertyCounts_Creat}{RGB}{240,223,178}
\definecolor{colorCommonVoice17PropertyCounts_Creat}{RGB}{245,242,234}
\definecolor{colorCoNASEPropertyCounts_Creat}{RGB}{240,223,178}
\definecolor{colorNigerianEnglishPropertyCounts_Creat}{RGB}{240,223,178}
\definecolor{colorNorwegianParl.SpeechPropertyCounts_Creat}{RGB}{240,223,178}
\definecolor{color120hSpanishSpeechPropertyCounts_Creat}{RGB}{240,223,178}
\definecolor{colorDiDiSpeechPropertyCounts_Creat}{RGB}{240,223,178}
\definecolor{colorCzechParliamentPropertyCounts_Creat}{RGB}{240,223,178}
\definecolor{colorCoVoST-2PropertyCounts_Creat}{RGB}{240,223,178}
\definecolor{colorKSCPropertyCounts_Creat}{RGB}{240,223,178}
\definecolor{colorBasq.,Cat.andGal.PropertyCounts_Creat}{RGB}{240,223,178}
\definecolor{colorKsponSpeechPropertyCounts_Creat}{RGB}{240,223,178}
\definecolor{colorSamromurPropertyCounts_Creat}{RGB}{240,223,178}
\definecolor{colorMultiling.LibriSpeechPropertyCounts_Creat}{RGB}{240,223,178}
\definecolor{colorMaSSPropertyCounts_Creat}{RGB}{240,223,178}
\definecolor{colorFTSPEECHPropertyCounts_Creat}{RGB}{245,237,214}
\definecolor{colorEng.Acc.inBrit.IslesPropertyCounts_Creat}{RGB}{240,223,178}
\definecolor{colorHighlandPueblaNahuatlPropertyCounts_Creat}{RGB}{245,242,234}
\definecolor{colorQASRPropertyCounts_Creat}{RGB}{245,237,214}
\definecolor{colorMultiling.TEDxPropertyCounts_Creat}{RGB}{245,242,234}
\definecolor{colorMinds14PropertyCounts_Creat}{RGB}{240,223,178}
\definecolor{colorGolosPropertyCounts_Creat}{RGB}{245,242,234}
\definecolor{colorMASCPropertyCounts_Creat}{RGB}{245,242,234}
\definecolor{colorLaboroTVSpeechPropertyCounts_Creat}{RGB}{245,237,214}
\definecolor{colorKeSpeechPropertyCounts_Creat}{RGB}{240,223,178}
\definecolor{colorJTUBESPEECHPropertyCounts_Creat}{RGB}{242,244,244}
\definecolor{colorGigaSpeechPropertyCounts_Creat}{RGB}{206,235,231}
\definecolor{colorVoxPopuliPropertyCounts_Creat}{RGB}{240,223,178}
\definecolor{colorSPGISpeechPropertyCounts_Creat}{RGB}{242,244,244}
\definecolor{colorWestAfr.RadioPropertyCounts_Creat}{RGB}{245,237,214}
\definecolor{colorAISHELL-4PropertyCounts_Creat}{RGB}{242,244,244}
\definecolor{colorWestAfr.Virt.Asst.PropertyCounts_Creat}{RGB}{245,237,214}
\definecolor{colorMediaSpeechPropertyCounts_Creat}{RGB}{231,241,240}
\definecolor{colorPeople'sSpeechPropertyCounts_Creat}{RGB}{217,238,235}
\definecolor{color1111HoursHindiPropertyCounts_Creat}{RGB}{240,223,178}
\definecolor{colorShrutilipiPropertyCounts_Creat}{RGB}{245,237,214}
\definecolor{colorWenetSpeechPropertyCounts_Creat}{RGB}{242,244,244}
\definecolor{colorSamromurChildrenPropertyCounts_Creat}{RGB}{240,223,178}
\definecolor{colorSDS-200PropertyCounts_Creat}{RGB}{245,242,234}
\definecolor{coloraidatatangPropertyCounts_Creat}{RGB}{240,223,178}
\definecolor{colorFleursPropertyCounts_Creat}{RGB}{245,242,234}
\definecolor{colorOLKAVSPropertyCounts_Creat}{RGB}{245,237,214}
\definecolor{colorNorwegianParl.PropertyCounts_Creat}{RGB}{245,237,214}
\definecolor{colorMagicData-RAMCPropertyCounts_Creat}{RGB}{242,244,244}
\definecolor{colorKathbathPropertyCounts_Creat}{RGB}{245,237,214}
\definecolor{colorHebrewKanPropertyCounts_Creat}{RGB}{240,223,178}
\definecolor{colorHebrewCourseraPropertyCounts_Creat}{RGB}{240,223,178}
\definecolor{colorBloomSpeechPropertyCounts_Creat}{RGB}{231,241,240}
\definecolor{colorEnglish-VietnamesePropertyCounts_Creat}{RGB}{240,223,178}
\definecolor{colorEarnings-22PropertyCounts_Creat}{RGB}{240,223,178}
\definecolor{colorYODASPropertyCounts_Creat}{RGB}{245,242,234}
\definecolor{colorAFRISPEECH-200PropertyCounts_Creat}{RGB}{179,226,219}
\definecolor{colorAaltoFinnishParl.PropertyCounts_Creat}{RGB}{240,223,178}
\definecolor{colorReazonSpeechPropertyCounts_Creat}{RGB}{245,237,214}
\definecolor{colorEdAccPropertyCounts_Creat}{RGB}{240,223,178}
\definecolor{colorRixVoxPropertyCounts_Creat}{RGB}{240,223,178}
\definecolor{colorJapaneseAnimeSpeechPropertyCounts_Creat}{RGB}{240,223,178}
\definecolor{colorSnowMountainPropertyCounts_Creat}{RGB}{245,237,214}
\definecolor{colorSamromurMilljonPropertyCounts_Creat}{RGB}{240,223,178}
\definecolor{colorBud500PropertyCounts_Creat}{RGB}{240,223,178}
\definecolor{colorVibraVoxPropertyCounts_Creat}{RGB}{240,223,178}
\definecolor{colorM2ASRPropertyCounts_Creat}{RGB}{245,242,234}
\definecolor{colorTIMITPropertyCounts_Tasks}{RGB}{245,242,234}
\definecolor{colorSwitchboardPropertyCounts_Tasks}{RGB}{240,223,178}
\definecolor{colorAfricanAcc.FrenchPropertyCounts_Tasks}{RGB}{240,223,178}
\definecolor{colorCSJPropertyCounts_Tasks}{RGB}{240,223,178}
\definecolor{colorFisherPropertyCounts_Tasks}{RGB}{240,223,178}
\definecolor{colorCSLU22Langs.PropertyCounts_Tasks}{RGB}{240,223,178}
\definecolor{colorAMIPropertyCounts_Tasks}{RGB}{240,223,178}
\definecolor{colorCSLU1.2PropertyCounts_Tasks}{RGB}{240,223,178}
\definecolor{colorALLSSTARPropertyCounts_Tasks}{RGB}{240,223,178}
\definecolor{colorTED-LIUM3PropertyCounts_Tasks}{RGB}{245,237,214}
\definecolor{colorNSTNorwegianPropertyCounts_Tasks}{RGB}{240,223,178}
\definecolor{colorNSTDanishPropertyCounts_Tasks}{RGB}{240,223,178}
\definecolor{colorNSTSwedishPropertyCounts_Tasks}{RGB}{240,223,178}
\definecolor{colorVystadialPropertyCounts_Tasks}{RGB}{240,223,178}
\definecolor{colorTHCHS-30PropertyCounts_Tasks}{RGB}{240,223,178}
\definecolor{colorLibriSpeechPropertyCounts_Tasks}{RGB}{240,223,178}
\definecolor{colorTHUYG-20PropertyCounts_Tasks}{RGB}{245,237,214}
\definecolor{colorVCTKPropertyCounts_Tasks}{RGB}{240,223,178}
\definecolor{colorSpokenWikipediaPropertyCounts_Tasks}{RGB}{240,223,178}
\definecolor{colorAISHELL-1PropertyCounts_Tasks}{RGB}{245,237,214}
\definecolor{colorLJSpeechPropertyCounts_Tasks}{RGB}{240,223,178}
\definecolor{colorClarinPLPropertyCounts_Tasks}{RGB}{240,223,178}
\definecolor{colorAISHELL-2PropertyCounts_Tasks}{RGB}{245,237,214}
\definecolor{colorRegionalAf.Am.Lang.PropertyCounts_Tasks}{RGB}{240,223,178}
\definecolor{colorCrowdSourcedSpeechPropertyCounts_Tasks}{RGB}{240,223,178}
\definecolor{colorZeroth-KoreanPropertyCounts_Tasks}{RGB}{240,223,178}
\definecolor{colorRTVEPropertyCounts_Tasks}{RGB}{240,223,178}
\definecolor{colorOpenSTTPropertyCounts_Tasks}{RGB}{245,237,214}
\definecolor{colorMuST-CPropertyCounts_Tasks}{RGB}{245,237,214}
\definecolor{colorM-AILABSPropertyCounts_Tasks}{RGB}{240,223,178}
\definecolor{colorMAGICDATAPropertyCounts_Tasks}{RGB}{240,223,178}
\definecolor{colorCommonVoice17PropertyCounts_Tasks}{RGB}{245,242,234}
\definecolor{colorCoNASEPropertyCounts_Tasks}{RGB}{240,223,178}
\definecolor{colorNigerianEnglishPropertyCounts_Tasks}{RGB}{240,223,178}
\definecolor{colorNorwegianParl.SpeechPropertyCounts_Tasks}{RGB}{240,223,178}
\definecolor{color120hSpanishSpeechPropertyCounts_Tasks}{RGB}{240,223,178}
\definecolor{colorDiDiSpeechPropertyCounts_Tasks}{RGB}{240,223,178}
\definecolor{colorCzechParliamentPropertyCounts_Tasks}{RGB}{240,223,178}
\definecolor{colorCoVoST-2PropertyCounts_Tasks}{RGB}{240,223,178}
\definecolor{colorKSCPropertyCounts_Tasks}{RGB}{240,223,178}
\definecolor{colorBasq.,Cat.andGal.PropertyCounts_Tasks}{RGB}{240,223,178}
\definecolor{colorKsponSpeechPropertyCounts_Tasks}{RGB}{240,223,178}
\definecolor{colorSamromurPropertyCounts_Tasks}{RGB}{240,223,178}
\definecolor{colorMultiling.LibriSpeechPropertyCounts_Tasks}{RGB}{240,223,178}
\definecolor{colorMaSSPropertyCounts_Tasks}{RGB}{240,223,178}
\definecolor{colorFTSPEECHPropertyCounts_Tasks}{RGB}{245,237,214}
\definecolor{colorEng.Acc.inBrit.IslesPropertyCounts_Tasks}{RGB}{240,223,178}
\definecolor{colorHighlandPueblaNahuatlPropertyCounts_Tasks}{RGB}{245,242,234}
\definecolor{colorQASRPropertyCounts_Tasks}{RGB}{245,237,214}
\definecolor{colorMultiling.TEDxPropertyCounts_Tasks}{RGB}{245,242,234}
\definecolor{colorMinds14PropertyCounts_Tasks}{RGB}{240,223,178}
\definecolor{colorGolosPropertyCounts_Tasks}{RGB}{245,242,234}
\definecolor{colorMASCPropertyCounts_Tasks}{RGB}{245,242,234}
\definecolor{colorLaboroTVSpeechPropertyCounts_Tasks}{RGB}{245,237,214}
\definecolor{colorKeSpeechPropertyCounts_Tasks}{RGB}{240,223,178}
\definecolor{colorJTUBESPEECHPropertyCounts_Tasks}{RGB}{242,244,244}
\definecolor{colorGigaSpeechPropertyCounts_Tasks}{RGB}{206,235,231}
\definecolor{colorVoxPopuliPropertyCounts_Tasks}{RGB}{240,223,178}
\definecolor{colorSPGISpeechPropertyCounts_Tasks}{RGB}{242,244,244}
\definecolor{colorWestAfr.RadioPropertyCounts_Tasks}{RGB}{245,237,214}
\definecolor{colorAISHELL-4PropertyCounts_Tasks}{RGB}{242,244,244}
\definecolor{colorWestAfr.Virt.Asst.PropertyCounts_Tasks}{RGB}{245,237,214}
\definecolor{colorMediaSpeechPropertyCounts_Tasks}{RGB}{231,241,240}
\definecolor{colorPeople'sSpeechPropertyCounts_Tasks}{RGB}{217,238,235}
\definecolor{color1111HoursHindiPropertyCounts_Tasks}{RGB}{240,223,178}
\definecolor{colorShrutilipiPropertyCounts_Tasks}{RGB}{245,237,214}
\definecolor{colorWenetSpeechPropertyCounts_Tasks}{RGB}{242,244,244}
\definecolor{colorSamromurChildrenPropertyCounts_Tasks}{RGB}{240,223,178}
\definecolor{colorSDS-200PropertyCounts_Tasks}{RGB}{245,242,234}
\definecolor{coloraidatatangPropertyCounts_Tasks}{RGB}{240,223,178}
\definecolor{colorFleursPropertyCounts_Tasks}{RGB}{245,242,234}
\definecolor{colorOLKAVSPropertyCounts_Tasks}{RGB}{245,237,214}
\definecolor{colorNorwegianParl.PropertyCounts_Tasks}{RGB}{245,237,214}
\definecolor{colorMagicData-RAMCPropertyCounts_Tasks}{RGB}{242,244,244}
\definecolor{colorKathbathPropertyCounts_Tasks}{RGB}{245,237,214}
\definecolor{colorHebrewKanPropertyCounts_Tasks}{RGB}{240,223,178}
\definecolor{colorHebrewCourseraPropertyCounts_Tasks}{RGB}{240,223,178}
\definecolor{colorBloomSpeechPropertyCounts_Tasks}{RGB}{231,241,240}
\definecolor{colorEnglish-VietnamesePropertyCounts_Tasks}{RGB}{240,223,178}
\definecolor{colorEarnings-22PropertyCounts_Tasks}{RGB}{240,223,178}
\definecolor{colorYODASPropertyCounts_Tasks}{RGB}{245,242,234}
\definecolor{colorAFRISPEECH-200PropertyCounts_Tasks}{RGB}{179,226,219}
\definecolor{colorAaltoFinnishParl.PropertyCounts_Tasks}{RGB}{240,223,178}
\definecolor{colorReazonSpeechPropertyCounts_Tasks}{RGB}{245,237,214}
\definecolor{colorEdAccPropertyCounts_Tasks}{RGB}{240,223,178}
\definecolor{colorRixVoxPropertyCounts_Tasks}{RGB}{240,223,178}
\definecolor{colorJapaneseAnimeSpeechPropertyCounts_Tasks}{RGB}{240,223,178}
\definecolor{colorSnowMountainPropertyCounts_Tasks}{RGB}{245,237,214}
\definecolor{colorSamromurMilljonPropertyCounts_Tasks}{RGB}{240,223,178}
\definecolor{colorBud500PropertyCounts_Tasks}{RGB}{240,223,178}
\definecolor{colorVibraVoxPropertyCounts_Tasks}{RGB}{240,223,178}
\definecolor{colorM2ASRPropertyCounts_Tasks}{RGB}{245,242,234}
\definecolor{colorTIMITPropertyCounts_Src}{RGB}{240,223,178}
\definecolor{colorSwitchboardPropertyCounts_Src}{RGB}{240,223,178}
\definecolor{colorAfricanAcc.FrenchPropertyCounts_Src}{RGB}{240,223,178}
\definecolor{colorCSJPropertyCounts_Src}{RGB}{240,223,178}
\definecolor{colorFisherPropertyCounts_Src}{RGB}{240,223,178}
\definecolor{colorCSLU22Langs.PropertyCounts_Src}{RGB}{240,223,178}
\definecolor{colorAMIPropertyCounts_Src}{RGB}{245,237,216}
\definecolor{colorCSLU1.2PropertyCounts_Src}{RGB}{240,223,178}
\definecolor{colorALLSSTARPropertyCounts_Src}{RGB}{240,223,178}
\definecolor{colorTED-LIUM3PropertyCounts_Src}{RGB}{240,223,178}
\definecolor{colorNSTNorwegianPropertyCounts_Src}{RGB}{240,223,178}
\definecolor{colorNSTDanishPropertyCounts_Src}{RGB}{240,223,178}
\definecolor{colorNSTSwedishPropertyCounts_Src}{RGB}{240,223,178}
\definecolor{colorVystadialPropertyCounts_Src}{RGB}{245,237,216}
\definecolor{colorTHCHS-30PropertyCounts_Src}{RGB}{240,223,178}
\definecolor{colorLibriSpeechPropertyCounts_Src}{RGB}{240,223,178}
\definecolor{colorTHUYG-20PropertyCounts_Src}{RGB}{240,223,178}
\definecolor{colorVCTKPropertyCounts_Src}{RGB}{240,223,178}
\definecolor{colorSpokenWikipediaPropertyCounts_Src}{RGB}{240,223,178}
\definecolor{colorAISHELL-1PropertyCounts_Src}{RGB}{245,237,216}
\definecolor{colorLJSpeechPropertyCounts_Src}{RGB}{240,223,178}
\definecolor{colorClarinPLPropertyCounts_Src}{RGB}{245,237,216}
\definecolor{colorAISHELL-2PropertyCounts_Src}{RGB}{240,223,178}
\definecolor{colorRegionalAf.Am.Lang.PropertyCounts_Src}{RGB}{240,223,178}
\definecolor{colorCrowdSourcedSpeechPropertyCounts_Src}{RGB}{240,223,178}
\definecolor{colorZeroth-KoreanPropertyCounts_Src}{RGB}{240,223,178}
\definecolor{colorRTVEPropertyCounts_Src}{RGB}{240,223,178}
\definecolor{colorOpenSTTPropertyCounts_Src}{RGB}{245,237,216}
\definecolor{colorMuST-CPropertyCounts_Src}{RGB}{240,223,178}
\definecolor{colorM-AILABSPropertyCounts_Src}{RGB}{240,223,178}
\definecolor{colorMAGICDATAPropertyCounts_Src}{RGB}{240,223,178}
\definecolor{colorCommonVoice17PropertyCounts_Src}{RGB}{240,223,178}
\definecolor{colorCoNASEPropertyCounts_Src}{RGB}{240,223,178}
\definecolor{colorNigerianEnglishPropertyCounts_Src}{RGB}{240,223,178}
\definecolor{colorNorwegianParl.SpeechPropertyCounts_Src}{RGB}{240,223,178}
\definecolor{color120hSpanishSpeechPropertyCounts_Src}{RGB}{240,223,178}
\definecolor{colorDiDiSpeechPropertyCounts_Src}{RGB}{240,223,178}
\definecolor{colorCzechParliamentPropertyCounts_Src}{RGB}{240,223,178}
\definecolor{colorCoVoST-2PropertyCounts_Src}{RGB}{245,237,216}
\definecolor{colorKSCPropertyCounts_Src}{RGB}{240,223,178}
\definecolor{colorBasq.,Cat.andGal.PropertyCounts_Src}{RGB}{240,223,178}
\definecolor{colorKsponSpeechPropertyCounts_Src}{RGB}{240,223,178}
\definecolor{colorSamromurPropertyCounts_Src}{RGB}{240,223,178}
\definecolor{colorMultiling.LibriSpeechPropertyCounts_Src}{RGB}{240,223,178}
\definecolor{colorMaSSPropertyCounts_Src}{RGB}{240,223,178}
\definecolor{colorFTSPEECHPropertyCounts_Src}{RGB}{240,223,178}
\definecolor{colorEng.Acc.inBrit.IslesPropertyCounts_Src}{RGB}{240,223,178}
\definecolor{colorHighlandPueblaNahuatlPropertyCounts_Src}{RGB}{240,223,178}
\definecolor{colorQASRPropertyCounts_Src}{RGB}{240,223,178}
\definecolor{colorMultiling.TEDxPropertyCounts_Src}{RGB}{240,223,178}
\definecolor{colorMinds14PropertyCounts_Src}{RGB}{245,237,216}
\definecolor{colorGolosPropertyCounts_Src}{RGB}{240,223,178}
\definecolor{colorMASCPropertyCounts_Src}{RGB}{240,223,178}
\definecolor{colorLaboroTVSpeechPropertyCounts_Src}{RGB}{240,223,178}
\definecolor{colorKeSpeechPropertyCounts_Src}{RGB}{240,223,178}
\definecolor{colorJTUBESPEECHPropertyCounts_Src}{RGB}{240,223,178}
\definecolor{colorGigaSpeechPropertyCounts_Src}{RGB}{245,243,238}
\definecolor{colorVoxPopuliPropertyCounts_Src}{RGB}{240,223,178}
\definecolor{colorSPGISpeechPropertyCounts_Src}{RGB}{240,223,178}
\definecolor{colorWestAfr.RadioPropertyCounts_Src}{RGB}{240,223,178}
\definecolor{colorAISHELL-4PropertyCounts_Src}{RGB}{245,237,216}
\definecolor{colorWestAfr.Virt.Asst.PropertyCounts_Src}{RGB}{240,223,178}
\definecolor{colorMediaSpeechPropertyCounts_Src}{RGB}{179,226,219}
\definecolor{colorPeople'sSpeechPropertyCounts_Src}{RGB}{245,237,216}
\definecolor{color1111HoursHindiPropertyCounts_Src}{RGB}{240,223,178}
\definecolor{colorShrutilipiPropertyCounts_Src}{RGB}{240,223,178}
\definecolor{colorWenetSpeechPropertyCounts_Src}{RGB}{245,237,216}
\definecolor{colorSamromurChildrenPropertyCounts_Src}{RGB}{240,223,178}
\definecolor{colorSDS-200PropertyCounts_Src}{RGB}{240,223,178}
\definecolor{coloraidatatangPropertyCounts_Src}{RGB}{240,223,178}
\definecolor{colorFleursPropertyCounts_Src}{RGB}{240,223,178}
\definecolor{colorOLKAVSPropertyCounts_Src}{RGB}{240,223,178}
\definecolor{colorNorwegianParl.PropertyCounts_Src}{RGB}{240,223,178}
\definecolor{colorMagicData-RAMCPropertyCounts_Src}{RGB}{240,223,178}
\definecolor{colorKathbathPropertyCounts_Src}{RGB}{240,223,178}
\definecolor{colorHebrewKanPropertyCounts_Src}{RGB}{240,223,178}
\definecolor{colorHebrewCourseraPropertyCounts_Src}{RGB}{240,223,178}
\definecolor{colorBloomSpeechPropertyCounts_Src}{RGB}{240,223,178}
\definecolor{colorEnglish-VietnamesePropertyCounts_Src}{RGB}{240,223,178}
\definecolor{colorEarnings-22PropertyCounts_Src}{RGB}{245,243,238}
\definecolor{colorYODASPropertyCounts_Src}{RGB}{240,223,178}
\definecolor{colorAFRISPEECH-200PropertyCounts_Src}{RGB}{240,223,178}
\definecolor{colorAaltoFinnishParl.PropertyCounts_Src}{RGB}{240,223,178}
\definecolor{colorReazonSpeechPropertyCounts_Src}{RGB}{240,223,178}
\definecolor{colorEdAccPropertyCounts_Src}{RGB}{240,223,178}
\definecolor{colorRixVoxPropertyCounts_Src}{RGB}{240,223,178}
\definecolor{colorJapaneseAnimeSpeechPropertyCounts_Src}{RGB}{240,223,178}
\definecolor{colorSnowMountainPropertyCounts_Src}{RGB}{240,223,178}
\definecolor{colorSamromurMilljonPropertyCounts_Src}{RGB}{240,223,178}
\definecolor{colorBud500PropertyCounts_Src}{RGB}{245,237,216}
\definecolor{colorVibraVoxPropertyCounts_Src}{RGB}{240,223,178}
\definecolor{colorM2ASRPropertyCounts_Src}{RGB}{240,223,178}
\definecolor{colorTIMITPropertyCounts_Top}{RGB}{245,242,234}
\definecolor{colorSwitchboardPropertyCounts_Top}{RGB}{196,232,227}
\definecolor{colorAfricanAcc.FrenchPropertyCounts_Top}{RGB}{245,242,234}
\definecolor{colorCSJPropertyCounts_Top}{RGB}{245,233,200}
\definecolor{colorFisherPropertyCounts_Top}{RGB}{213,237,234}
\definecolor{colorCSLU22Langs.PropertyCounts_Top}{RGB}{245,242,234}
\definecolor{colorAMIPropertyCounts_Top}{RGB}{245,233,200}
\definecolor{colorCSLU1.2PropertyCounts_Top}{RGB}{240,223,178}
\definecolor{colorALLSSTARPropertyCounts_Top}{RGB}{245,236,212}
\definecolor{colorTED-LIUM3PropertyCounts_Top}{RGB}{240,223,178}
\definecolor{colorNSTNorwegianPropertyCounts_Top}{RGB}{245,242,234}
\definecolor{colorNSTDanishPropertyCounts_Top}{RGB}{245,242,234}
\definecolor{colorNSTSwedishPropertyCounts_Top}{RGB}{245,242,234}
\definecolor{colorVystadialPropertyCounts_Top}{RGB}{245,236,212}
\definecolor{colorTHCHS-30PropertyCounts_Top}{RGB}{240,223,178}
\definecolor{colorLibriSpeechPropertyCounts_Top}{RGB}{179,226,219}
\definecolor{colorTHUYG-20PropertyCounts_Top}{RGB}{245,236,212}
\definecolor{colorVCTKPropertyCounts_Top}{RGB}{240,223,178}
\definecolor{colorSpokenWikipediaPropertyCounts_Top}{RGB}{240,223,178}
\definecolor{colorAISHELL-1PropertyCounts_Top}{RGB}{244,244,244}
\definecolor{colorLJSpeechPropertyCounts_Top}{RGB}{240,223,178}
\definecolor{colorClarinPLPropertyCounts_Top}{RGB}{245,242,234}
\definecolor{colorAISHELL-2PropertyCounts_Top}{RGB}{245,243,238}
\definecolor{colorRegionalAf.Am.Lang.PropertyCounts_Top}{RGB}{245,243,238}
\definecolor{colorCrowdSourcedSpeechPropertyCounts_Top}{RGB}{240,223,178}
\definecolor{colorZeroth-KoreanPropertyCounts_Top}{RGB}{245,242,234}
\definecolor{colorRTVEPropertyCounts_Top}{RGB}{245,242,234}
\definecolor{colorOpenSTTPropertyCounts_Top}{RGB}{245,241,230}
\definecolor{colorMuST-CPropertyCounts_Top}{RGB}{245,238,220}
\definecolor{colorM-AILABSPropertyCounts_Top}{RGB}{217,238,235}
\definecolor{colorMAGICDATAPropertyCounts_Top}{RGB}{240,223,178}
\definecolor{colorCommonVoice17PropertyCounts_Top}{RGB}{240,223,178}
\definecolor{colorCoNASEPropertyCounts_Top}{RGB}{245,241,230}
\definecolor{colorNigerianEnglishPropertyCounts_Top}{RGB}{245,242,234}
\definecolor{colorNorwegianParl.SpeechPropertyCounts_Top}{RGB}{245,242,234}
\definecolor{color120hSpanishSpeechPropertyCounts_Top}{RGB}{245,242,234}
\definecolor{colorDiDiSpeechPropertyCounts_Top}{RGB}{245,233,200}
\definecolor{colorCzechParliamentPropertyCounts_Top}{RGB}{245,242,234}
\definecolor{colorCoVoST-2PropertyCounts_Top}{RGB}{240,223,178}
\definecolor{colorKSCPropertyCounts_Top}{RGB}{245,240,226}
\definecolor{colorBasq.,Cat.andGal.PropertyCounts_Top}{RGB}{245,233,200}
\definecolor{colorKsponSpeechPropertyCounts_Top}{RGB}{245,241,230}
\definecolor{colorSamromurPropertyCounts_Top}{RGB}{245,240,226}
\definecolor{colorMultiling.LibriSpeechPropertyCounts_Top}{RGB}{217,238,235}
\definecolor{colorMaSSPropertyCounts_Top}{RGB}{240,223,178}
\definecolor{colorFTSPEECHPropertyCounts_Top}{RGB}{245,233,200}
\definecolor{colorEng.Acc.inBrit.IslesPropertyCounts_Top}{RGB}{245,238,220}
\definecolor{colorHighlandPueblaNahuatlPropertyCounts_Top}{RGB}{245,242,234}
\definecolor{colorQASRPropertyCounts_Top}{RGB}{245,242,234}
\definecolor{colorMultiling.TEDxPropertyCounts_Top}{RGB}{245,242,234}
\definecolor{colorMinds14PropertyCounts_Top}{RGB}{245,242,234}
\definecolor{colorGolosPropertyCounts_Top}{RGB}{245,241,230}
\definecolor{colorMASCPropertyCounts_Top}{RGB}{235,242,241}
\definecolor{colorLaboroTVSpeechPropertyCounts_Top}{RGB}{245,242,234}
\definecolor{colorKeSpeechPropertyCounts_Top}{RGB}{240,223,178}
\definecolor{colorJTUBESPEECHPropertyCounts_Top}{RGB}{245,242,234}
\definecolor{colorGigaSpeechPropertyCounts_Top}{RGB}{224,240,237}
\definecolor{colorVoxPopuliPropertyCounts_Top}{RGB}{240,223,178}
\definecolor{colorSPGISpeechPropertyCounts_Top}{RGB}{245,233,200}
\definecolor{colorWestAfr.RadioPropertyCounts_Top}{RGB}{245,236,212}
\definecolor{colorAISHELL-4PropertyCounts_Top}{RGB}{245,241,230}
\definecolor{colorWestAfr.Virt.Asst.PropertyCounts_Top}{RGB}{245,233,200}
\definecolor{colorMediaSpeechPropertyCounts_Top}{RGB}{240,223,178}
\definecolor{colorPeople'sSpeechPropertyCounts_Top}{RGB}{236,243,242}
\definecolor{color1111HoursHindiPropertyCounts_Top}{RGB}{245,240,226}
\definecolor{colorShrutilipiPropertyCounts_Top}{RGB}{240,223,178}
\definecolor{colorWenetSpeechPropertyCounts_Top}{RGB}{245,244,244}
\definecolor{colorSamromurChildrenPropertyCounts_Top}{RGB}{245,240,226}
\definecolor{colorSDS-200PropertyCounts_Top}{RGB}{245,233,200}
\definecolor{coloraidatatangPropertyCounts_Top}{RGB}{245,242,234}
\definecolor{colorFleursPropertyCounts_Top}{RGB}{244,244,244}
\definecolor{colorOLKAVSPropertyCounts_Top}{RGB}{236,243,242}
\definecolor{colorNorwegianParl.PropertyCounts_Top}{RGB}{245,233,200}
\definecolor{colorMagicData-RAMCPropertyCounts_Top}{RGB}{235,242,241}
\definecolor{colorKathbathPropertyCounts_Top}{RGB}{245,236,212}
\definecolor{colorHebrewKanPropertyCounts_Top}{RGB}{245,236,212}
\definecolor{colorHebrewCourseraPropertyCounts_Top}{RGB}{245,242,234}
\definecolor{colorBloomSpeechPropertyCounts_Top}{RGB}{245,243,238}
\definecolor{colorEnglish-VietnamesePropertyCounts_Top}{RGB}{245,242,234}
\definecolor{colorEarnings-22PropertyCounts_Top}{RGB}{245,233,200}
\definecolor{colorYODASPropertyCounts_Top}{RGB}{240,223,178}
\definecolor{colorAFRISPEECH-200PropertyCounts_Top}{RGB}{245,241,230}
\definecolor{colorAaltoFinnishParl.PropertyCounts_Top}{RGB}{245,233,200}
\definecolor{colorReazonSpeechPropertyCounts_Top}{RGB}{240,223,178}
\definecolor{colorEdAccPropertyCounts_Top}{RGB}{245,243,238}
\definecolor{colorRixVoxPropertyCounts_Top}{RGB}{245,233,200}
\definecolor{colorJapaneseAnimeSpeechPropertyCounts_Top}{RGB}{245,242,234}
\definecolor{colorSnowMountainPropertyCounts_Top}{RGB}{240,223,178}
\definecolor{colorSamromurMilljonPropertyCounts_Top}{RGB}{245,240,226}
\definecolor{colorBud500PropertyCounts_Top}{RGB}{245,238,220}
\definecolor{colorVibraVoxPropertyCounts_Top}{RGB}{240,223,178}
\definecolor{colorM2ASRPropertyCounts_Top}{RGB}{245,244,242}

% [inline block 0: 1 envs, 45314 chars -> data_tex | \begin{longtable}{lc|ccccccc|ccc|c} \caption[\textbf{Audio collections and properties}]{\textbf{Audio collections and pr...]


\setlength{\tabcolsep}{1.9pt}
\definecolor{colorHOLLYWOOD2PropertyCounts_Hours}{RGB}{229,241,239}
\definecolor{colorCollectivePropertyCounts_Hours}{RGB}{240,223,178}
\definecolor{colorHMDBPropertyCounts_Hours}{RGB}{204,235,230}
\definecolor{colorUCF101PropertyCounts_Hours}{RGB}{227,240,239}
\definecolor{color50SaladsPropertyCounts_Hours}{RGB}{226,240,238}
\definecolor{colorYouCookPropertyCounts_Hours}{RGB}{213,237,234}
\definecolor{colorVideoStoryPropertyCounts_Hours}{RGB}{213,237,234}
\definecolor{colorHollywoodExt.PropertyCounts_Hours}{RGB}{233,242,240}
\definecolor{colorTHUMOSPropertyCounts_Hours}{RGB}{218,238,235}
\definecolor{colorBreakfastPropertyCounts_Hours}{RGB}{224,240,237}
\definecolor{colorSumMePropertyCounts_Hours}{RGB}{242,244,244}
\definecolor{colorSports-1MPropertyCounts_Hours}{RGB}{187,229,223}
\definecolor{colorStoryGraphsPropertyCounts_Hours}{RGB}{235,242,241}
\definecolor{colorTVSumPropertyCounts_Hours}{RGB}{236,243,242}
\definecolor{colorVolleyballPropertyCounts_Hours}{RGB}{240,223,178}
\definecolor{colorActivityNetPropertyCounts_Hours}{RGB}{213,237,234}
\definecolor{colorMovieQAPropertyCounts_Hours}{RGB}{217,238,235}
\definecolor{colorCharadesPropertyCounts_Hours}{RGB}{224,240,237}
\definecolor{colorMarsPropertyCounts_Hours}{RGB}{240,223,178}
\definecolor{colorMSR-VTTPropertyCounts_Hours}{RGB}{226,240,238}
\definecolor{colorVTWPropertyCounts_Hours}{RGB}{218,238,235}
\definecolor{colorTGIFPropertyCounts_Hours}{RGB}{224,240,237}
\definecolor{colorNTURGB+DPropertyCounts_Hours}{RGB}{224,240,237}
\definecolor{colorNarratedInstr.Vid.PropertyCounts_Hours}{RGB}{235,242,241}
\definecolor{colorYoutube-8MPropertyCounts_Hours}{RGB}{179,226,219}
\definecolor{colorYouCook2PropertyCounts_Hours}{RGB}{220,239,236}
\definecolor{colorMultiTHUMOSPropertyCounts_Hours}{RGB}{227,240,239}
\definecolor{colorImageNet-VidPropertyCounts_Hours}{RGB}{233,242,240}
\definecolor{colorPKU-MMDPropertyCounts_Hours}{RGB}{226,240,238}
\definecolor{color20BN-SOMETHINGPropertyCounts_Hours}{RGB}{222,239,237}
\definecolor{colorVoxCelebPropertyCounts_Hours}{RGB}{209,236,232}
\definecolor{colorQFVSPropertyCounts_Hours}{RGB}{229,241,239}
\definecolor{colorDavisPropertyCounts_Hours}{RGB}{240,223,178}
\definecolor{colorDiDeMoPropertyCounts_Hours}{RGB}{218,238,235}
\definecolor{colorHow2PropertyCounts_Hours}{RGB}{209,236,232}
\definecolor{colorSOAPropertyCounts_Hours}{RGB}{211,237,233}
\definecolor{colorVLOGPropertyCounts_Hours}{RGB}{217,238,235}
\definecolor{colorCharades-EgoPropertyCounts_Hours}{RGB}{224,240,237}
\definecolor{colorEPIC-KITCHENSPropertyCounts_Hours}{RGB}{222,239,237}
\definecolor{colorMovieGraphsPropertyCounts_Hours}{RGB}{222,239,237}
\definecolor{color20BN-jesterPropertyCounts_Hours}{RGB}{231,241,240}
\definecolor{colorCOINPropertyCounts_Hours}{RGB}{215,237,234}
\definecolor{colorCrossTaskPropertyCounts_Hours}{RGB}{217,238,235}
\definecolor{colorToyotaSmarthomePropertyCounts_Hours}{RGB}{218,238,235}
\definecolor{colorVaTeXPropertyCounts_Hours}{RGB}{222,239,237}
\definecolor{colorMSAPropertyCounts_Hours}{RGB}{215,237,234}
\definecolor{colorMMActPropertyCounts_Hours}{RGB}{222,239,237}
\definecolor{colorTRECVidPropertyCounts_Hours}{RGB}{213,237,234}
\definecolor{colorHACSPropertyCounts_Hours}{RGB}{213,237,234}
\definecolor{colorHowTo100MPropertyCounts_Hours}{RGB}{187,229,223}
\definecolor{colorMomentsinTimePropertyCounts_Hours}{RGB}{213,237,234}
\definecolor{colorVIOLINPropertyCounts_Hours}{RGB}{215,237,234}
\definecolor{colorTITANPropertyCounts_Hours}{RGB}{238,243,242}
\definecolor{colorRareActPropertyCounts_Hours}{RGB}{229,241,239}
\definecolor{colorTinyVIRATPropertyCounts_Hours}{RGB}{231,241,240}
\definecolor{color100DOHPropertyCounts_Hours}{RGB}{206,235,231}
\definecolor{colorOops!PropertyCounts_Hours}{RGB}{226,240,238}
\definecolor{colorOmniSource-WebPropertyCounts_Hours}{RGB}{200,234,229}
\definecolor{colorCondensedMoviesPropertyCounts_Hours}{RGB}{211,237,233}
\definecolor{colorMovieScenesPropertyCounts_Hours}{RGB}{218,238,235}
\definecolor{colorMovie-NetPropertyCounts_Hours}{RGB}{208,236,232}
\definecolor{colorEEVPropertyCounts_Hours}{RGB}{217,238,235}
\definecolor{colorFineGymPropertyCounts_Hours}{RGB}{213,237,234}
\definecolor{colorLEMMAPropertyCounts_Hours}{RGB}{231,241,240}
\definecolor{colorHAA500PropertyCounts_Hours}{RGB}{235,242,241}
\definecolor{colorHVUPropertyCounts_Hours}{RGB}{190,230,224}
\definecolor{colorApesPropertyCounts_Hours}{RGB}{227,240,239}
\definecolor{colorWebVidPropertyCounts_Hours}{RGB}{200,234,229}
\definecolor{colorVideoLTPropertyCounts_Hours}{RGB}{200,234,229}
\definecolor{colorUAV-HumanPropertyCounts_Hours}{RGB}{229,241,239}
\definecolor{colorHD-VILA-100MPropertyCounts_Hours}{RGB}{217,238,235}
\definecolor{colorHOMAGEPropertyCounts_Hours}{RGB}{227,240,239}
\definecolor{colorSpokenMomentsPropertyCounts_Hours}{RGB}{217,238,235}
\definecolor{colorM-MiTPropertyCounts_Hours}{RGB}{213,237,234}
\definecolor{colorQuerYDPropertyCounts_Hours}{RGB}{218,238,235}
\definecolor{colorMimeticsPropertyCounts_Hours}{RGB}{242,244,244}
\definecolor{colorFERV39kPropertyCounts_Hours}{RGB}{231,241,240}
\definecolor{colorMADPropertyCounts_Hours}{RGB}{211,237,233}
\definecolor{colorCDADPropertyCounts_Hours}{RGB}{218,238,235}
\definecolor{colorKineticsPropertyCounts_Hours}{RGB}{206,235,231}
\definecolor{colorLSMDCPropertyCounts_Hours}{RGB}{217,238,235}
\definecolor{colorEgo4DPropertyCounts_Hours}{RGB}{206,235,231}
\definecolor{colorMPIIPropertyCounts_Hours}{RGB}{222,239,237}
\definecolor{colorAvaPropertyCounts_Hours}{RGB}{220,239,236}
\definecolor{colorProject-AriaPropertyCounts_Hours}{RGB}{211,237,233}
\definecolor{colorHOLLYWOOD2PropertyCounts_Datasets}{RGB}{240,223,178}
\definecolor{colorCollectivePropertyCounts_Datasets}{RGB}{240,223,178}
\definecolor{colorHMDBPropertyCounts_Datasets}{RGB}{240,223,178}
\definecolor{colorUCF101PropertyCounts_Datasets}{RGB}{240,223,178}
\definecolor{color50SaladsPropertyCounts_Datasets}{RGB}{240,223,178}
\definecolor{colorYouCookPropertyCounts_Datasets}{RGB}{240,223,178}
\definecolor{colorVideoStoryPropertyCounts_Datasets}{RGB}{240,223,178}
\definecolor{colorHollywoodExt.PropertyCounts_Datasets}{RGB}{240,223,178}
\definecolor{colorTHUMOSPropertyCounts_Datasets}{RGB}{240,223,178}
\definecolor{colorBreakfastPropertyCounts_Datasets}{RGB}{240,223,178}
\definecolor{colorSumMePropertyCounts_Datasets}{RGB}{240,223,178}
\definecolor{colorSports-1MPropertyCounts_Datasets}{RGB}{240,223,178}
\definecolor{colorStoryGraphsPropertyCounts_Datasets}{RGB}{240,223,178}
\definecolor{colorTVSumPropertyCounts_Datasets}{RGB}{240,223,178}
\definecolor{colorVolleyballPropertyCounts_Datasets}{RGB}{240,223,178}
\definecolor{colorActivityNetPropertyCounts_Datasets}{RGB}{240,223,178}
\definecolor{colorMovieQAPropertyCounts_Datasets}{RGB}{240,223,178}
\definecolor{colorCharadesPropertyCounts_Datasets}{RGB}{240,223,178}
\definecolor{colorMarsPropertyCounts_Datasets}{RGB}{240,223,178}
\definecolor{colorMSR-VTTPropertyCounts_Datasets}{RGB}{240,223,178}
\definecolor{colorVTWPropertyCounts_Datasets}{RGB}{240,223,178}
\definecolor{colorTGIFPropertyCounts_Datasets}{RGB}{240,223,178}
\definecolor{colorNTURGB+DPropertyCounts_Datasets}{RGB}{240,223,178}
\definecolor{colorNarratedInstr.Vid.PropertyCounts_Datasets}{RGB}{240,223,178}
\definecolor{colorYoutube-8MPropertyCounts_Datasets}{RGB}{240,223,178}
\definecolor{colorYouCook2PropertyCounts_Datasets}{RGB}{240,223,178}
\definecolor{colorMultiTHUMOSPropertyCounts_Datasets}{RGB}{240,223,178}
\definecolor{colorImageNet-VidPropertyCounts_Datasets}{RGB}{240,223,178}
\definecolor{colorPKU-MMDPropertyCounts_Datasets}{RGB}{240,223,178}
\definecolor{color20BN-SOMETHINGPropertyCounts_Datasets}{RGB}{240,223,178}
\definecolor{colorVoxCelebPropertyCounts_Datasets}{RGB}{240,223,178}
\definecolor{colorQFVSPropertyCounts_Datasets}{RGB}{240,223,178}
\definecolor{colorDavisPropertyCounts_Datasets}{RGB}{240,223,178}
\definecolor{colorDiDeMoPropertyCounts_Datasets}{RGB}{240,223,178}
\definecolor{colorHow2PropertyCounts_Datasets}{RGB}{240,223,178}
\definecolor{colorSOAPropertyCounts_Datasets}{RGB}{240,223,178}
\definecolor{colorVLOGPropertyCounts_Datasets}{RGB}{240,223,178}
\definecolor{colorCharades-EgoPropertyCounts_Datasets}{RGB}{240,223,178}
\definecolor{colorEPIC-KITCHENSPropertyCounts_Datasets}{RGB}{240,223,178}
\definecolor{colorMovieGraphsPropertyCounts_Datasets}{RGB}{240,223,178}
\definecolor{color20BN-jesterPropertyCounts_Datasets}{RGB}{240,223,178}
\definecolor{colorCOINPropertyCounts_Datasets}{RGB}{240,223,178}
\definecolor{colorCrossTaskPropertyCounts_Datasets}{RGB}{240,223,178}
\definecolor{colorToyotaSmarthomePropertyCounts_Datasets}{RGB}{240,223,178}
\definecolor{colorVaTeXPropertyCounts_Datasets}{RGB}{240,223,178}
\definecolor{colorMSAPropertyCounts_Datasets}{RGB}{240,223,178}
\definecolor{colorMMActPropertyCounts_Datasets}{RGB}{240,223,178}
\definecolor{colorTRECVidPropertyCounts_Datasets}{RGB}{240,223,178}
\definecolor{colorHACSPropertyCounts_Datasets}{RGB}{240,223,178}
\definecolor{colorHowTo100MPropertyCounts_Datasets}{RGB}{240,223,178}
\definecolor{colorMomentsinTimePropertyCounts_Datasets}{RGB}{240,223,178}
\definecolor{colorVIOLINPropertyCounts_Datasets}{RGB}{240,223,178}
\definecolor{colorTITANPropertyCounts_Datasets}{RGB}{240,223,178}
\definecolor{colorRareActPropertyCounts_Datasets}{RGB}{240,223,178}
\definecolor{colorTinyVIRATPropertyCounts_Datasets}{RGB}{240,223,178}
\definecolor{color100DOHPropertyCounts_Datasets}{RGB}{240,223,178}
\definecolor{colorOops!PropertyCounts_Datasets}{RGB}{240,223,178}
\definecolor{colorOmniSource-WebPropertyCounts_Datasets}{RGB}{240,223,178}
\definecolor{colorCondensedMoviesPropertyCounts_Datasets}{RGB}{240,223,178}
\definecolor{colorMovieScenesPropertyCounts_Datasets}{RGB}{240,223,178}
\definecolor{colorMovie-NetPropertyCounts_Datasets}{RGB}{240,223,178}
\definecolor{colorEEVPropertyCounts_Datasets}{RGB}{240,223,178}
\definecolor{colorFineGymPropertyCounts_Datasets}{RGB}{240,223,178}
\definecolor{colorLEMMAPropertyCounts_Datasets}{RGB}{240,223,178}
\definecolor{colorHAA500PropertyCounts_Datasets}{RGB}{240,223,178}
\definecolor{colorHVUPropertyCounts_Datasets}{RGB}{240,223,178}
\definecolor{colorApesPropertyCounts_Datasets}{RGB}{240,223,178}
\definecolor{colorWebVidPropertyCounts_Datasets}{RGB}{240,223,178}
\definecolor{colorVideoLTPropertyCounts_Datasets}{RGB}{240,223,178}
\definecolor{colorUAV-HumanPropertyCounts_Datasets}{RGB}{240,223,178}
\definecolor{colorHD-VILA-100MPropertyCounts_Datasets}{RGB}{240,223,178}
\definecolor{colorHOMAGEPropertyCounts_Datasets}{RGB}{240,223,178}
\definecolor{colorSpokenMomentsPropertyCounts_Datasets}{RGB}{240,223,178}
\definecolor{colorM-MiTPropertyCounts_Datasets}{RGB}{240,223,178}
\definecolor{colorQuerYDPropertyCounts_Datasets}{RGB}{240,223,178}
\definecolor{colorMimeticsPropertyCounts_Datasets}{RGB}{240,223,178}
\definecolor{colorFERV39kPropertyCounts_Datasets}{RGB}{240,223,178}
\definecolor{colorMADPropertyCounts_Datasets}{RGB}{240,223,178}
\definecolor{colorCDADPropertyCounts_Datasets}{RGB}{240,223,178}
\definecolor{colorKineticsPropertyCounts_Datasets}{RGB}{179,226,219}
\definecolor{colorLSMDCPropertyCounts_Datasets}{RGB}{229,241,239}
\definecolor{colorEgo4DPropertyCounts_Datasets}{RGB}{229,241,239}
\definecolor{colorMPIIPropertyCounts_Datasets}{RGB}{179,226,219}
\definecolor{colorAvaPropertyCounts_Datasets}{RGB}{229,241,239}
\definecolor{colorProject-AriaPropertyCounts_Datasets}{RGB}{229,241,239}
\definecolor{colorHOLLYWOOD2PropertyCounts_Countries}{RGB}{239,221,175}
\definecolor{colorCollectivePropertyCounts_Countries}{RGB}{239,221,175}
\definecolor{colorHMDBPropertyCounts_Countries}{RGB}{245,244,244}
\definecolor{colorUCF101PropertyCounts_Countries}{RGB}{239,221,175}
\definecolor{color50SaladsPropertyCounts_Countries}{RGB}{239,221,175}
\definecolor{colorYouCookPropertyCounts_Countries}{RGB}{239,221,175}
\definecolor{colorVideoStoryPropertyCounts_Countries}{RGB}{239,221,175}
\definecolor{colorHollywoodExt.PropertyCounts_Countries}{RGB}{239,221,175}
\definecolor{colorTHUMOSPropertyCounts_Countries}{RGB}{245,244,244}
\definecolor{colorBreakfastPropertyCounts_Countries}{RGB}{245,244,244}
\definecolor{colorSumMePropertyCounts_Countries}{RGB}{245,244,244}
\definecolor{colorSports-1MPropertyCounts_Countries}{RGB}{239,221,175}
\definecolor{colorStoryGraphsPropertyCounts_Countries}{RGB}{239,221,175}
\definecolor{colorTVSumPropertyCounts_Countries}{RGB}{239,221,175}
\definecolor{colorVolleyballPropertyCounts_Countries}{RGB}{239,221,175}
\definecolor{colorActivityNetPropertyCounts_Countries}{RGB}{245,244,244}
\definecolor{colorMovieQAPropertyCounts_Countries}{RGB}{211,237,233}
\definecolor{colorCharadesPropertyCounts_Countries}{RGB}{245,244,244}
\definecolor{colorMarsPropertyCounts_Countries}{RGB}{239,221,175}
\definecolor{colorMSR-VTTPropertyCounts_Countries}{RGB}{239,221,175}
\definecolor{colorVTWPropertyCounts_Countries}{RGB}{245,244,244}
\definecolor{colorTGIFPropertyCounts_Countries}{RGB}{239,221,175}
\definecolor{colorNTURGB+DPropertyCounts_Countries}{RGB}{239,221,175}
\definecolor{colorNarratedInstr.Vid.PropertyCounts_Countries}{RGB}{245,244,244}
\definecolor{colorYoutube-8MPropertyCounts_Countries}{RGB}{239,221,175}
\definecolor{colorYouCook2PropertyCounts_Countries}{RGB}{239,221,175}
\definecolor{colorMultiTHUMOSPropertyCounts_Countries}{RGB}{245,244,244}
\definecolor{colorImageNet-VidPropertyCounts_Countries}{RGB}{239,221,175}
\definecolor{colorPKU-MMDPropertyCounts_Countries}{RGB}{239,221,175}
\definecolor{color20BN-SOMETHINGPropertyCounts_Countries}{RGB}{239,221,175}
\definecolor{colorVoxCelebPropertyCounts_Countries}{RGB}{245,244,244}
\definecolor{colorQFVSPropertyCounts_Countries}{RGB}{239,221,175}
\definecolor{colorDavisPropertyCounts_Countries}{RGB}{239,221,175}
\definecolor{colorDiDeMoPropertyCounts_Countries}{RGB}{239,221,175}
\definecolor{colorHow2PropertyCounts_Countries}{RGB}{239,221,175}
\definecolor{colorSOAPropertyCounts_Countries}{RGB}{239,221,175}
\definecolor{colorVLOGPropertyCounts_Countries}{RGB}{239,221,175}
\definecolor{colorCharades-EgoPropertyCounts_Countries}{RGB}{239,221,175}
\definecolor{colorEPIC-KITCHENSPropertyCounts_Countries}{RGB}{211,237,233}
\definecolor{colorMovieGraphsPropertyCounts_Countries}{RGB}{239,221,175}
\definecolor{color20BN-jesterPropertyCounts_Countries}{RGB}{239,221,175}
\definecolor{colorCOINPropertyCounts_Countries}{RGB}{239,221,175}
\definecolor{colorCrossTaskPropertyCounts_Countries}{RGB}{179,226,219}
\definecolor{colorToyotaSmarthomePropertyCounts_Countries}{RGB}{239,221,175}
\definecolor{colorVaTeXPropertyCounts_Countries}{RGB}{245,244,244}
\definecolor{colorMSAPropertyCounts_Countries}{RGB}{245,244,244}
\definecolor{colorMMActPropertyCounts_Countries}{RGB}{245,244,244}
\definecolor{colorTRECVidPropertyCounts_Countries}{RGB}{239,221,175}
\definecolor{colorHACSPropertyCounts_Countries}{RGB}{239,221,175}
\definecolor{colorHowTo100MPropertyCounts_Countries}{RGB}{245,244,244}
\definecolor{colorMomentsinTimePropertyCounts_Countries}{RGB}{239,221,175}
\definecolor{colorVIOLINPropertyCounts_Countries}{RGB}{239,221,175}
\definecolor{colorTITANPropertyCounts_Countries}{RGB}{239,221,175}
\definecolor{colorRareActPropertyCounts_Countries}{RGB}{211,237,233}
\definecolor{colorTinyVIRATPropertyCounts_Countries}{RGB}{239,221,175}
\definecolor{color100DOHPropertyCounts_Countries}{RGB}{239,221,175}
\definecolor{colorOops!PropertyCounts_Countries}{RGB}{239,221,175}
\definecolor{colorOmniSource-WebPropertyCounts_Countries}{RGB}{239,221,175}
\definecolor{colorCondensedMoviesPropertyCounts_Countries}{RGB}{239,221,175}
\definecolor{colorMovieScenesPropertyCounts_Countries}{RGB}{245,244,244}
\definecolor{colorMovie-NetPropertyCounts_Countries}{RGB}{239,221,175}
\definecolor{colorEEVPropertyCounts_Countries}{RGB}{239,221,175}
\definecolor{colorFineGymPropertyCounts_Countries}{RGB}{239,221,175}
\definecolor{colorLEMMAPropertyCounts_Countries}{RGB}{239,221,175}
\definecolor{colorHAA500PropertyCounts_Countries}{RGB}{245,244,244}
\definecolor{colorHVUPropertyCounts_Countries}{RGB}{211,237,233}
\definecolor{colorApesPropertyCounts_Countries}{RGB}{211,237,233}
\definecolor{colorWebVidPropertyCounts_Countries}{RGB}{245,244,244}
\definecolor{colorVideoLTPropertyCounts_Countries}{RGB}{245,244,244}
\definecolor{colorUAV-HumanPropertyCounts_Countries}{RGB}{245,244,244}
\definecolor{colorHD-VILA-100MPropertyCounts_Countries}{RGB}{239,221,175}
\definecolor{colorHOMAGEPropertyCounts_Countries}{RGB}{239,221,175}
\definecolor{colorSpokenMomentsPropertyCounts_Countries}{RGB}{239,221,175}
\definecolor{colorM-MiTPropertyCounts_Countries}{RGB}{239,221,175}
\definecolor{colorQuerYDPropertyCounts_Countries}{RGB}{239,221,175}
\definecolor{colorMimeticsPropertyCounts_Countries}{RGB}{239,221,175}
\definecolor{colorFERV39kPropertyCounts_Countries}{RGB}{239,221,175}
\definecolor{colorMADPropertyCounts_Countries}{RGB}{239,221,175}
\definecolor{colorCDADPropertyCounts_Countries}{RGB}{239,221,175}
\definecolor{colorKineticsPropertyCounts_Countries}{RGB}{239,221,175}
\definecolor{colorLSMDCPropertyCounts_Countries}{RGB}{179,226,219}
\definecolor{colorEgo4DPropertyCounts_Countries}{RGB}{239,221,175}
\definecolor{colorMPIIPropertyCounts_Countries}{RGB}{239,221,175}
\definecolor{colorAvaPropertyCounts_Countries}{RGB}{239,221,175}
\definecolor{colorProject-AriaPropertyCounts_Countries}{RGB}{239,221,175}
\definecolor{colorHOLLYWOOD2PropertyCounts_Creators}{RGB}{240,223,178}
\definecolor{colorCollectivePropertyCounts_Creators}{RGB}{240,223,178}
\definecolor{colorHMDBPropertyCounts_Creators}{RGB}{245,244,242}
\definecolor{colorUCF101PropertyCounts_Creators}{RGB}{240,223,178}
\definecolor{color50SaladsPropertyCounts_Creators}{RGB}{240,223,178}
\definecolor{colorYouCookPropertyCounts_Creators}{RGB}{240,223,178}
\definecolor{colorVideoStoryPropertyCounts_Creators}{RGB}{240,223,178}
\definecolor{colorHollywoodExt.PropertyCounts_Creators}{RGB}{240,223,178}
\definecolor{colorTHUMOSPropertyCounts_Creators}{RGB}{233,242,240}
\definecolor{colorBreakfastPropertyCounts_Creators}{RGB}{245,238,220}
\definecolor{colorSumMePropertyCounts_Creators}{RGB}{245,244,242}
\definecolor{colorSports-1MPropertyCounts_Creators}{RGB}{240,223,178}
\definecolor{colorStoryGraphsPropertyCounts_Creators}{RGB}{240,223,178}
\definecolor{colorTVSumPropertyCounts_Creators}{RGB}{240,223,178}
\definecolor{colorVolleyballPropertyCounts_Creators}{RGB}{240,223,178}
\definecolor{colorActivityNetPropertyCounts_Creators}{RGB}{245,238,220}
\definecolor{colorMovieQAPropertyCounts_Creators}{RGB}{245,244,242}
\definecolor{colorCharadesPropertyCounts_Creators}{RGB}{233,242,240}
\definecolor{colorMarsPropertyCounts_Creators}{RGB}{233,242,240}
\definecolor{colorMSR-VTTPropertyCounts_Creators}{RGB}{240,223,178}
\definecolor{colorVTWPropertyCounts_Creators}{RGB}{245,238,220}
\definecolor{colorTGIFPropertyCounts_Creators}{RGB}{245,244,242}
\definecolor{colorNTURGB+DPropertyCounts_Creators}{RGB}{240,223,178}
\definecolor{colorNarratedInstr.Vid.PropertyCounts_Creators}{RGB}{233,242,240}
\definecolor{colorYoutube-8MPropertyCounts_Creators}{RGB}{240,223,178}
\definecolor{colorYouCook2PropertyCounts_Creators}{RGB}{245,238,220}
\definecolor{colorMultiTHUMOSPropertyCounts_Creators}{RGB}{245,244,242}
\definecolor{colorImageNet-VidPropertyCounts_Creators}{RGB}{240,223,178}
\definecolor{colorPKU-MMDPropertyCounts_Creators}{RGB}{245,238,220}
\definecolor{color20BN-SOMETHINGPropertyCounts_Creators}{RGB}{240,223,178}
\definecolor{colorVoxCelebPropertyCounts_Creators}{RGB}{240,223,178}
\definecolor{colorQFVSPropertyCounts_Creators}{RGB}{245,238,220}
\definecolor{colorDavisPropertyCounts_Creators}{RGB}{245,238,220}
\definecolor{colorDiDeMoPropertyCounts_Creators}{RGB}{240,223,178}
\definecolor{colorHow2PropertyCounts_Creators}{RGB}{240,223,178}
\definecolor{colorSOAPropertyCounts_Creators}{RGB}{240,223,178}
\definecolor{colorVLOGPropertyCounts_Creators}{RGB}{240,223,178}
\definecolor{colorCharades-EgoPropertyCounts_Creators}{RGB}{240,223,178}
\definecolor{colorEPIC-KITCHENSPropertyCounts_Creators}{RGB}{245,244,242}
\definecolor{colorMovieGraphsPropertyCounts_Creators}{RGB}{245,244,242}
\definecolor{color20BN-jesterPropertyCounts_Creators}{RGB}{240,223,178}
\definecolor{colorCOINPropertyCounts_Creators}{RGB}{245,238,220}
\definecolor{colorCrossTaskPropertyCounts_Creators}{RGB}{222,239,237}
\definecolor{colorToyotaSmarthomePropertyCounts_Creators}{RGB}{240,223,178}
\definecolor{colorVaTeXPropertyCounts_Creators}{RGB}{245,238,220}
\definecolor{colorMSAPropertyCounts_Creators}{RGB}{245,238,220}
\definecolor{colorMMActPropertyCounts_Creators}{RGB}{245,238,220}
\definecolor{colorTRECVidPropertyCounts_Creators}{RGB}{240,223,178}
\definecolor{colorHACSPropertyCounts_Creators}{RGB}{245,244,242}
\definecolor{colorHowTo100MPropertyCounts_Creators}{RGB}{233,242,240}
\definecolor{colorMomentsinTimePropertyCounts_Creators}{RGB}{240,223,178}
\definecolor{colorVIOLINPropertyCounts_Creators}{RGB}{240,223,178}
\definecolor{colorTITANPropertyCounts_Creators}{RGB}{240,223,178}
\definecolor{colorRareActPropertyCounts_Creators}{RGB}{222,239,237}
\definecolor{colorTinyVIRATPropertyCounts_Creators}{RGB}{240,223,178}
\definecolor{color100DOHPropertyCounts_Creators}{RGB}{245,238,220}
\definecolor{colorOops!PropertyCounts_Creators}{RGB}{240,223,178}
\definecolor{colorOmniSource-WebPropertyCounts_Creators}{RGB}{240,223,178}
\definecolor{colorCondensedMoviesPropertyCounts_Creators}{RGB}{240,223,178}
\definecolor{colorMovieScenesPropertyCounts_Creators}{RGB}{245,238,220}
\definecolor{colorMovie-NetPropertyCounts_Creators}{RGB}{240,223,178}
\definecolor{colorEEVPropertyCounts_Creators}{RGB}{245,238,220}
\definecolor{colorFineGymPropertyCounts_Creators}{RGB}{240,223,178}
\definecolor{colorLEMMAPropertyCounts_Creators}{RGB}{240,223,178}
\definecolor{colorHAA500PropertyCounts_Creators}{RGB}{233,242,240}
\definecolor{colorHVUPropertyCounts_Creators}{RGB}{222,239,237}
\definecolor{colorApesPropertyCounts_Creators}{RGB}{245,244,242}
\definecolor{colorWebVidPropertyCounts_Creators}{RGB}{245,238,220}
\definecolor{colorVideoLTPropertyCounts_Creators}{RGB}{233,242,240}
\definecolor{colorUAV-HumanPropertyCounts_Creators}{RGB}{245,238,220}
\definecolor{colorHD-VILA-100MPropertyCounts_Creators}{RGB}{240,223,178}
\definecolor{colorHOMAGEPropertyCounts_Creators}{RGB}{245,238,220}
\definecolor{colorSpokenMomentsPropertyCounts_Creators}{RGB}{245,244,242}
\definecolor{colorM-MiTPropertyCounts_Creators}{RGB}{240,223,178}
\definecolor{colorQuerYDPropertyCounts_Creators}{RGB}{240,223,178}
\definecolor{colorMimeticsPropertyCounts_Creators}{RGB}{240,223,178}
\definecolor{colorFERV39kPropertyCounts_Creators}{RGB}{240,223,178}
\definecolor{colorMADPropertyCounts_Creators}{RGB}{240,223,178}
\definecolor{colorCDADPropertyCounts_Creators}{RGB}{245,238,220}
\definecolor{colorKineticsPropertyCounts_Creators}{RGB}{240,223,178}
\definecolor{colorLSMDCPropertyCounts_Creators}{RGB}{179,226,219}
\definecolor{colorEgo4DPropertyCounts_Creators}{RGB}{245,238,220}
\definecolor{colorMPIIPropertyCounts_Creators}{RGB}{245,238,220}
\definecolor{colorAvaPropertyCounts_Creators}{RGB}{240,223,178}
\definecolor{colorProject-AriaPropertyCounts_Creators}{RGB}{240,223,178}
\definecolor{colorHOLLYWOOD2PropertyCounts_Sources}{RGB}{240,223,178}
\definecolor{colorCollectivePropertyCounts_Sources}{RGB}{240,223,178}
\definecolor{colorHMDBPropertyCounts_Sources}{RGB}{226,240,238}
\definecolor{colorUCF101PropertyCounts_Sources}{RGB}{240,223,178}
\definecolor{color50SaladsPropertyCounts_Sources}{RGB}{240,223,178}
\definecolor{colorYouCookPropertyCounts_Sources}{RGB}{240,223,178}
\definecolor{colorVideoStoryPropertyCounts_Sources}{RGB}{240,223,178}
\definecolor{colorHollywoodExt.PropertyCounts_Sources}{RGB}{240,223,178}
\definecolor{colorTHUMOSPropertyCounts_Sources}{RGB}{240,223,178}
\definecolor{colorBreakfastPropertyCounts_Sources}{RGB}{240,223,178}
\definecolor{colorSumMePropertyCounts_Sources}{RGB}{240,223,178}
\definecolor{colorSports-1MPropertyCounts_Sources}{RGB}{240,223,178}
\definecolor{colorStoryGraphsPropertyCounts_Sources}{RGB}{240,223,178}
\definecolor{colorTVSumPropertyCounts_Sources}{RGB}{240,223,178}
\definecolor{colorVolleyballPropertyCounts_Sources}{RGB}{240,223,178}
\definecolor{colorActivityNetPropertyCounts_Sources}{RGB}{240,223,178}
\definecolor{colorMovieQAPropertyCounts_Sources}{RGB}{240,223,178}
\definecolor{colorCharadesPropertyCounts_Sources}{RGB}{240,223,178}
\definecolor{colorMarsPropertyCounts_Sources}{RGB}{240,223,178}
\definecolor{colorMSR-VTTPropertyCounts_Sources}{RGB}{240,223,178}
\definecolor{colorVTWPropertyCounts_Sources}{RGB}{240,223,178}
\definecolor{colorTGIFPropertyCounts_Sources}{RGB}{240,223,178}
\definecolor{colorNTURGB+DPropertyCounts_Sources}{RGB}{240,223,178}
\definecolor{colorNarratedInstr.Vid.PropertyCounts_Sources}{RGB}{240,223,178}
\definecolor{colorYoutube-8MPropertyCounts_Sources}{RGB}{240,223,178}
\definecolor{colorYouCook2PropertyCounts_Sources}{RGB}{240,223,178}
\definecolor{colorMultiTHUMOSPropertyCounts_Sources}{RGB}{240,223,178}
\definecolor{colorImageNet-VidPropertyCounts_Sources}{RGB}{240,223,178}
\definecolor{colorPKU-MMDPropertyCounts_Sources}{RGB}{240,223,178}
\definecolor{color20BN-SOMETHINGPropertyCounts_Sources}{RGB}{240,223,178}
\definecolor{colorVoxCelebPropertyCounts_Sources}{RGB}{240,223,178}
\definecolor{colorQFVSPropertyCounts_Sources}{RGB}{240,223,178}
\definecolor{colorDavisPropertyCounts_Sources}{RGB}{240,223,178}
\definecolor{colorDiDeMoPropertyCounts_Sources}{RGB}{240,223,178}
\definecolor{colorHow2PropertyCounts_Sources}{RGB}{240,223,178}
\definecolor{colorSOAPropertyCounts_Sources}{RGB}{240,223,178}
\definecolor{colorVLOGPropertyCounts_Sources}{RGB}{240,223,178}
\definecolor{colorCharades-EgoPropertyCounts_Sources}{RGB}{240,223,178}
\definecolor{colorEPIC-KITCHENSPropertyCounts_Sources}{RGB}{240,223,178}
\definecolor{colorMovieGraphsPropertyCounts_Sources}{RGB}{240,223,178}
\definecolor{color20BN-jesterPropertyCounts_Sources}{RGB}{240,223,178}
\definecolor{colorCOINPropertyCounts_Sources}{RGB}{240,223,178}
\definecolor{colorCrossTaskPropertyCounts_Sources}{RGB}{240,223,178}
\definecolor{colorToyotaSmarthomePropertyCounts_Sources}{RGB}{240,223,178}
\definecolor{colorVaTeXPropertyCounts_Sources}{RGB}{240,223,178}
\definecolor{colorMSAPropertyCounts_Sources}{RGB}{240,223,178}
\definecolor{colorMMActPropertyCounts_Sources}{RGB}{240,223,178}
\definecolor{colorTRECVidPropertyCounts_Sources}{RGB}{245,238,218}
\definecolor{colorHACSPropertyCounts_Sources}{RGB}{240,223,178}
\definecolor{colorHowTo100MPropertyCounts_Sources}{RGB}{240,223,178}
\definecolor{colorMomentsinTimePropertyCounts_Sources}{RGB}{179,226,219}
\definecolor{colorVIOLINPropertyCounts_Sources}{RGB}{240,223,178}
\definecolor{colorTITANPropertyCounts_Sources}{RGB}{240,223,178}
\definecolor{colorRareActPropertyCounts_Sources}{RGB}{240,223,178}
\definecolor{colorTinyVIRATPropertyCounts_Sources}{RGB}{240,223,178}
\definecolor{color100DOHPropertyCounts_Sources}{RGB}{240,223,178}
\definecolor{colorOops!PropertyCounts_Sources}{RGB}{240,223,178}
\definecolor{colorOmniSource-WebPropertyCounts_Sources}{RGB}{245,243,240}
\definecolor{colorCondensedMoviesPropertyCounts_Sources}{RGB}{240,223,178}
\definecolor{colorMovieScenesPropertyCounts_Sources}{RGB}{240,223,178}
\definecolor{colorMovie-NetPropertyCounts_Sources}{RGB}{240,223,178}
\definecolor{colorEEVPropertyCounts_Sources}{RGB}{240,223,178}
\definecolor{colorFineGymPropertyCounts_Sources}{RGB}{240,223,178}
\definecolor{colorLEMMAPropertyCounts_Sources}{RGB}{245,238,218}
\definecolor{colorHAA500PropertyCounts_Sources}{RGB}{240,223,178}
\definecolor{colorHVUPropertyCounts_Sources}{RGB}{240,223,178}
\definecolor{colorApesPropertyCounts_Sources}{RGB}{240,223,178}
\definecolor{colorWebVidPropertyCounts_Sources}{RGB}{240,223,178}
\definecolor{colorVideoLTPropertyCounts_Sources}{RGB}{240,223,178}
\definecolor{colorUAV-HumanPropertyCounts_Sources}{RGB}{240,223,178}
\definecolor{colorHD-VILA-100MPropertyCounts_Sources}{RGB}{240,223,178}
\definecolor{colorHOMAGEPropertyCounts_Sources}{RGB}{240,223,178}
\definecolor{colorSpokenMomentsPropertyCounts_Sources}{RGB}{179,226,219}
\definecolor{colorM-MiTPropertyCounts_Sources}{RGB}{245,238,218}
\definecolor{colorQuerYDPropertyCounts_Sources}{RGB}{245,238,218}
\definecolor{colorMimeticsPropertyCounts_Sources}{RGB}{240,223,178}
\definecolor{colorFERV39kPropertyCounts_Sources}{RGB}{240,223,178}
\definecolor{colorMADPropertyCounts_Sources}{RGB}{240,223,178}
\definecolor{colorCDADPropertyCounts_Sources}{RGB}{240,223,178}
\definecolor{colorKineticsPropertyCounts_Sources}{RGB}{245,238,218}
\definecolor{colorLSMDCPropertyCounts_Sources}{RGB}{240,223,178}
\definecolor{colorEgo4DPropertyCounts_Sources}{RGB}{240,223,178}
\definecolor{colorMPIIPropertyCounts_Sources}{RGB}{245,238,218}
\definecolor{colorAvaPropertyCounts_Sources}{RGB}{245,238,218}
\definecolor{colorProject-AriaPropertyCounts_Sources}{RGB}{240,223,178}

% [inline block 1: 1 envs, 32843 chars -> data_tex | \begin{longtable}{lc|ccccc|cc} \caption[\textbf{Video collections and properties}]{\textbf{Video collections and propert...]


% \begingroup
% \renewcommand*{\arraystretch}{1.2}
% \input{tables/refs-licenses-text}
% \input{tables/refs-licenses-audio}
% \input{tables/refs-licenses-video}
% \endgroup
